# Supplementary material for: Inferring Epidemics from Multiple Dependent Data via Pseudo-Marginal Methods
Source: arXiv:2204.08901 ancillary file (2024-09-10)
Supplement: Supplementary file 1 [file SI_Corbella.pdf]

# Supplementary Information to Inferring epidemics from multiple dependent data via pseudo-marginal methods

A. Corbella, A. M. Presanis, P.J. Birrell, and D. De Angelis

March 31, 2022

## Contents

|          |                                                                                     |           |
|----------|-------------------------------------------------------------------------------------|-----------|
| <b>1</b> | <b>Analysis of dependent data</b>                                                   | <b>3</b>  |
| 1.1      | Estimation methodology . . . . .                                                    | 3         |
| 1.1.1    | Main sampling scheme . . . . .                                                      | 3         |
| 1.1.2    | Algorithms . . . . .                                                                | 4         |
| 1.1.3    | Choice between algorithms . . . . .                                                 | 5         |
| 1.2      | Results on the simulation study to assess the relevance of the dependence . . . . . | 6         |
| 1.2.1    | Comparison for transmission parameters . . . . .                                    | 6         |
| 1.2.2    | Results for transmission and severity parameters . . . . .                          | 9         |
| 1.2.3    | Influential parameters . . . . .                                                    | 12        |
| <b>2</b> | <b>Supplement to Section 5</b>                                                      | <b>12</b> |
| 2.1      | Model assumption . . . . .                                                          | 12        |
| 2.1.1    | Transmission and first severity layer . . . . .                                     | 12        |
| 2.1.2    | General Practitioner (GP)-consultations . . . . .                                   | 14        |
| 2.1.3    | Hospitalization and Intensive Care (IC) admissions . . . . .                        | 16        |
| 2.2      | Prior distributions . . . . .                                                       | 16        |
| 2.3      | Inference . . . . .                                                                 | 19        |
| 2.4      | Results . . . . .                                                                   | 19        |
| 2.4.1    | Transmission . . . . .                                                              | 19        |
| 2.4.2    | Severity . . . . .                                                                  | 20        |
| 2.4.3    | Background influenza-like illness (ILI) . . . . .                                   | 21        |
| 2.4.4    | Day-of-the-week effect . . . . .                                                    | 21        |
| 2.4.5    | Reporting . . . . .                                                                 | 22        |
| 2.4.6    | Goodness of fit . . . . .                                                           | 22        |

## List of Algorithms

|   |                                                  |   |
|---|--------------------------------------------------|---|
| 1 | First approximation of the likelihood . . . . .  | 4 |
| 2 | Second approximation of the likelihood . . . . . | 5 |

## List of Figures

|    |                                                                           |    |
|----|---------------------------------------------------------------------------|----|
| 1  | Comparison on transmission - small dependence (I) . . . . .               | 7  |
| 2  | Comparison on transmission - small dependence (II) . . . . .              | 7  |
| 3  | Comparison on transmission - big dependence (I) . . . . .                 | 8  |
| 4  | Comparison on transmission - big dependence (II) . . . . .                | 8  |
| 5  | Comparison on transmission and severity - small dependence (I) . . . . .  | 9  |
| 6  | Comparison on transmission and severity - small dependence (II) . . . . . | 10 |
| 7  | Comparison on transmission and severity - small dependence (I) . . . . .  | 11 |
| 8  | Comparison on transmission and severity - small dependence (II) . . . . . | 11 |
| 9  | Model directed acyclic graph (DAG). . . . .                               | 13 |
| 10 | Transmission parameters . . . . .                                         | 20 |
| 11 | Transmission summaries . . . . .                                          | 21 |
| 12 | Number of new infections . . . . .                                        | 22 |
| 13 | Severity parameters . . . . .                                             | 23 |
| 14 | Case GP consultation risk . . . . .                                       | 24 |
| 15 | Background ILI parameters . . . . .                                       | 24 |
| 16 | Background ILI trend . . . . .                                            | 25 |
| 17 | Day-of-the-week effect . . . . .                                          | 26 |
| 18 | Number of new infections . . . . .                                        | 26 |
| 19 | Shape paramtere of detection . . . . .                                    | 27 |
| 20 | Hospitalization detection . . . . .                                       | 27 |
| 21 | Goodness of fit GP data . . . . .                                         | 28 |
| 22 | Goodness of fit virology data . . . . .                                   | 29 |
| 23 | Goodness of fit hospital data . . . . .                                   | 30 |
| 24 | Goodness of fit ICU data . . . . .                                        | 31 |

## List of Tables

|   |                                                                                                         |    |
|---|---------------------------------------------------------------------------------------------------------|----|
| 1 | Pairwise comparison of variance - Small dependence . . . . .                                            | 7  |
| 2 | Pairwise comparison of variance - Big dependence . . . . .                                              | 8  |
| 3 | Pairwise comparison of variance - Small dependence; transmission and severity pa-<br>rameters . . . . . | 10 |
| 4 | Pairwise comparison of variance - Big dependence; transmission and severity param-<br>eters . . . . .   | 10 |
| 5 | Pairwise comparison of variance - Influential parameters . . . . .                                      | 12 |
| 6 | Prior distribution . . . . .                                                                            | 18 |

# 1 Analysis of dependent data

## 1.1 Estimation methodology

This section reports few results that lead to the construction and the choice of Algorithm 1 from the main text when inferring our proposed semi-stochastic model.

### 1.1.1 Main sampling scheme

Equations 9 and 10 of the main text model stochastic severity process as a chain of Binomial or Multinomial random variables (r.v.s) and Poisson r.v.s:

$$\begin{aligned}
({}^0X^H) &\sim \text{Pois}({}^0\xi \cdot {}^0\theta^H) \\
({}^0X_{t:t+D}^H | {}^0X_t^H = {}^0x_t^H) &\sim \text{Multi}({}_t^0x^H, {}^0f_{0:D}^H), & X_t^H &= \sum_{s=0}^S {}^0X_t^H \\
({}^HX_t^{\text{IC}} | X_t^H = x_t^H) &\sim \text{Bin}(x_t^H, {}^H\theta^{\text{IC}}) \\
({}^HX_{t:t+D}^{\text{IC}} | {}^HX_t^{\text{IC}} = {}^Hx_t^{\text{IC}}) &\sim \text{Multi}({}_t^Hx^{\text{IC}}, {}^Hf_{0:D}^{\text{IC}}), & X_t^{\text{IC}} &= \sum_{s=0}^S {}^HX_t^{\text{IC}} \\
(Y_t^H | X_t^H = x_t^H) &\sim \text{Bin}(x_t^H, \zeta_t^H) \\
(Y_t^{\text{IC}} | X_t^{\text{IC}} = x_t^{\text{IC}}) &\sim \text{Bin}(x_t^{\text{IC}}, \zeta_t^{\text{IC}})
\end{aligned}$$

for  $t = 0, 1, \dots, T$ .

Thanks to the Binomial-given-Poisson structure, it is straightforward to simulate from the hidden states given the observations deriving their posterior distribution for a general instance. Specifically, let:

$$\begin{aligned}
(X|\lambda) &\sim \text{Pois}(\lambda) \\
(Y|\theta, x) &\sim \text{Bin}(x, \theta) \\
(Y|\lambda, \theta) &\sim \text{Pois}(\lambda\theta), \quad \text{by property of the Poisson}
\end{aligned}$$

The distribution of  $X|y$  can be derived as follows:

$$\begin{aligned}
p(x|y) &= \frac{p(y|x)p(x)}{p(y)} && \text{by Bayes' theorem,} \\
&= \frac{\frac{x!}{y!(x-y)!} \theta^y (1-\theta)^{x-y} \frac{\lambda^x}{x!} e^{-\lambda}}{\frac{(\lambda\theta)^y}{y!} e^{-\lambda\theta}} \\
&= \frac{\lambda^{x-y} (1-\theta)^{x-y} e^{-\lambda(1-\theta)}}{\frac{1}{(x-y)!}}
\end{aligned}$$

which is the density function of a Poisson with rate  $\lambda(1-\theta)$  plus  $y$ . This recursion is heavily used in Algorithms 1 and 2 below.

### 1.1.2 Algorithms

The joint density of the dependent datasets can be factorised in two ways:

$$\begin{aligned} p(y_{1:T}^H, y_{1:T}^{IC} | \theta) &= p(y_{1:T}^H | y_{1:T}^{IC}, \theta) p(y_{1:T}^{IC} | \theta) \\ &= p(y_{1:T}^{IC} | y_{1:T}^H, \theta) p(y_{1:T}^H | \theta). \end{aligned}$$

Algorithm 1, reported in the main text, exploits the first decomposition, where  $p(y_{1:T}^{IC} | \theta)$  is available in closed form and a solution is needed for  $p(y_{1:T}^H | y_{1:T}^{IC}, \theta)$ , which is obtained by approximating the  $T$ -dimensional integral:

$$\begin{aligned} p(y_{1:T}^H | y_{1:T}^{IC}, \theta) &= \int_{X_1^H} \cdots \int_{X_T^H} p(y_{1:T}^H, X_{1:T}^H | y_{1:T}^{IC}, \theta) dX_1^H \cdots dX_T^H \\ &= \int_{X_1^H} \cdots \int_{X_T^H} p(y_{1:T}^H | X_{1:T}^H, y_{1:T}^{IC}, \theta) p(X_{1:T}^H | y_{1:T}^{IC}, \theta) dX_1^H \cdots dX_T^H \\ &= \int_{X_1^H} \cdots \int_{X_T^H} p(y_{1:T}^H | X_{1:T}^H, \theta) p(X_{1:T}^H | y_{1:T}^{IC}, \theta) dX_1^H \cdots dX_T^H \end{aligned}$$

by conditional independence of the state space model. The simulation of the hidden states is made simple by the distribution chosen for the severity and detection process.

**Result:**  $\hat{p}(y_{1:T}^H, y_{1:T}^{IC} | \theta)$

**Input:** fixed parameter  $\theta$ , number of particles  $N$ , data  $y_{1:T}^H, y_{1:T}^{IC}$

compute

$p(y_{1:T}^{IC} | \theta) = f(y_{1:T}^{IC} | \zeta_t^{IC} \cdot {}^H\theta^{IC} \cdot {}^0\theta^H \cdot \sum_{d=0}^D \sum_{g=0}^d \xi_{t-d-g}^0 \cdot {}^0f_d^H \cdot {}^Hf_g^{IC})$  with  $f(\cdot)$  being a Poisson density

**for**  $n = 1, \dots, N$  **do**

**for**  $t = 0, 1, \dots, T$  **do**

sample :  $x_t^{IC(n)} \sim \text{Pois}((1 - \zeta_t^{IC}) [{}^H\theta^{IC} \cdot {}^0\theta^H \sum_{d=0}^D \sum_{g=0}^d \xi_{t-d-g}^0 \cdot {}^0f_d^H \cdot {}^Hf_g^{IC}]) + y_T^{IC}$

sample :  ${}_{t-1}^H x_1^{IC(n)}, \dots, {}_{t-S}^H x_S^{IC(n)} \sim \text{Multi}(x_t^{IC(n)}, {}^Hf_{1:S}^{IC})$

compute :  ${}_{t-1}^H x_1^{IC(n)} = \sum_{s=1}^S {}_{t-s}^H x_s^{IC(n)}$

sample :  $x_t^{(n)} | {}_{t-1}^H x_1^{IC(n)}, \theta \sim \text{Pois}((1 - {}^H\theta^{IC}) [{}^0\theta^H \sum_{d=0}^D \xi_{t-d}^0 \cdot {}^0f_d^H]) + {}_{t-1}^H x_1^{IC(n)}$

**end**

compute :  $p(y_{1:T}^H | x_{1:T}^{(n)}, \theta) = g(y_{1:T}^H | x_{1:T}^{(n)}, \zeta_t^H)$  with  $g(\cdot)$  being a Binomial density

**end**

$\hat{p}(y_{1:T}^H, y_{1:T}^{IC} | \theta) = p(y_{1:T}^{IC} | \theta) \cdot \frac{1}{N} \sum_{n=1}^N p(y_{1:T}^H | x_{1:T}^{(n)}, \theta)$

**Algorithm 1:** First approximation of the likelihood

Algorithm 2 approximates the other factor.  $p(y_{1:T}^H | \theta)$  is available in closed form and a solution

is needed for  $p(y_{1:T}^{\text{IC}}|y_{1:T}^{\text{H}}, \boldsymbol{\theta})$ .

$$\begin{aligned} p(y_{1:T}^{\text{IC}}|y_{1:T}^{\text{H}}, \boldsymbol{\theta}) &= \int_{X_1^{\text{IC}}} \cdots \int_{X_T^{\text{IC}}} p(y_{1:T}^{\text{IC}}, X_{1:T}^{\text{IC}}|y_{1:T}^{\text{H}}, \boldsymbol{\theta}) dX_1^{\text{IC}} \cdots dX_T^{\text{IC}} \\ &= \int_{X_1^{\text{IC}}} \cdots \int_{X_T^{\text{IC}}} p(y_{1:T}^{\text{IC}}|X_{1:T}^{\text{IC}}, y_{1:T}^{\text{H}}, \boldsymbol{\theta}) p(X_{1:T}^{\text{IC}}|y_{1:T}^{\text{H}}, \boldsymbol{\theta}) dX_1^{\text{IC}} \cdots dX_T^{\text{IC}} \\ &= \int_{X_1^{\text{IC}}} \cdots \int_{X_T^{\text{IC}}} p(y_{1:T}^{\text{IC}}|X_{1:T}^{\text{IC}}, \boldsymbol{\theta}) p(X_{1:T}^{\text{IC}}|y_{1:T}^{\text{H}}, \boldsymbol{\theta}) dX_1^{\text{IC}} \cdots dX_T^{\text{IC}} \end{aligned}$$

**Result:**  $\hat{p}(y_{1:T}^{\text{H}}, y_{1:T}^{\text{IC}}|\boldsymbol{\theta})$   
**Input:**  $\boldsymbol{\theta}$ ,  $N$ ,  $y_{1:T}^{\text{H}}$ ,  $y_{1:T}^{\text{IC}}$   
compute  
 $p(y_{1:T}^{\text{H}}|\boldsymbol{\theta}) = f(y_{1:T}^{\text{H}}|\zeta_t^{\text{H}} \cdot {}^0\theta^{\text{H}} \cdot \sum_{d=0}^D \xi_{t-d}^0 \cdot {}^0f_d^{\text{H}})$  with  $f(\cdot)$  being a Poisson density  
**for**  $n = 1, \dots, N$  **do**  
    **for**  $t = 0, 1, \dots, T$  **do**  
        sample :  $x_t^{\text{H}(n)} \sim \text{Pois}((1 - \zeta_t^{\text{H}}) {}^0\theta^{\text{H}} \sum_{d=0}^D \xi_{t-d}^0 \cdot {}^0f_d^{\text{H}}) + y_t^{\text{H}}$   
        sample :  ${}_t^{\text{H}}x^{\text{IC}(n)}|x_t^{\text{H}(n)} \sim \text{Bin}(x_t^{\text{H}(n)}, {}^{\text{H}}\theta^{\text{IC}})$   
        sample :  ${}_t^{\text{H}}x_{1:S}^{\text{IC}(n)}|{}_t^{\text{H}}x^{\text{IC}(n)}, \boldsymbol{\theta} \sim \text{Multi}({}_t^{\text{H}}x^{\text{IC}(n)}, {}^{\text{H}}f_{1:S}^{\text{IC}})$   
        compute :  $x_t^{\text{IC}(n)} = \sum_{s=1}^S {}_t^{\text{H}}x_s^{\text{IC}(n)}$   
    **end**  
     $p(y_{1:T}^{\text{IC}}|x_{1:T}^{\text{IC}(n)}, \boldsymbol{\theta}) = g(y_{1:T}^{\text{IC}}|x_{1:T}^{\text{IC}(n)}, \zeta_t^{\text{IC}})$  with  $g(\cdot)$  being a Binomial density  
**end**  
 $\hat{p}(y_{1:T}^{\text{H}}, y_{1:T}^{\text{IC}}|\boldsymbol{\theta}) = p(y_{1:T}^{\text{H}}|\boldsymbol{\theta}) \cdot \frac{1}{N} \sum_{n=1}^N p(y_{1:T}^{\text{IC}}|x_{1:T}^{\text{IC}(n)}, \boldsymbol{\theta})$

**Algorithm 2:** Second approximation of the likelihood

### 1.1.3 Choice between algorithms

Both algorithms are very attractive since they use a vanilla Monte Carlo (MC) approximation. However, a better approximation can be obtained when the distribution from which the samples are drawn (in this case the distribution of the hidden states conditional on the first data included) matches well with the target distribution (in this case the distribution of the hidden states conditional on both) (Brooks et al., 2011). This matching improves substantially when the target distribution is more variable; in contrast, when the mass of the distribution is highly concentrated on a point, more simulations would result in low weights, hence they will be wasted. This principle motivates the choice between algorithm 1 and 2 as illustrated below.

For the case of UK Severe Influenza Surveillance System (USISS), as well as for many other observational collection schemes, more severe cases are monitored more carefully. While only approximately 20% of the hospitalised cases are recorded in the dataset, almost all IC cases are reported. The Binomial observational likelihood of  $y_{1:T}^{\text{H}}$  (Algorithm 1) is much more variable than the Binomial observational likelihood of  $y_{1:T}^{\text{IC}}$  (Algorithm 2). Moreover, the distribution from which

Algorithm 1 samples,  $x_{1:T}^H | y_{1:T}^{IC}$  results in 0 for all the sampled values  $x_t^{H(n)} < y_t^H$  for  $t = 1, \dots, T$ . Similarly the distribution from which Algorithm 2 samples,  $x_{1:T}^{IC} | y_{1:T}^H$  is equal to 0 for all the sampled values  $x_t^{IC(n)} < y_t^{IC}$  for  $t = 1, \dots, T$ . The latter case takes place much more often, due to the high detection of IC admissions: for this reason, obtaining a good sample for the MC approximation is much harder in this case. Hence Algorithm 1 is adopted in the main analysis.

## 1.2 Results on the simulation study to assess the relevance of the dependence

The setup and the comprehensive results from the simulation of Section 4 is presented below.

### 1.2.1 Comparison for transmission parameters

For the parameter inference with the approximated joint likelihood, a Monte Carlo within Metropolis (MCWM) algorithm with  $N = 2000$  was chosen. In fact, preliminary simulation experiments showed a much better mixing when the MCWM scheme was used in place of the grouped independence Metropolis Hastings (GIMH) and  $N = 2000$  was observed to be large enough to make the simulation study feasible and the bias of the MCWM algorithm negligible (i.e. to provide posterior distributions that were indistinguishable from the GIMH ones).

Hence, a MCWM algorithm including approximation of the joint likelihood via Algorithm 1 and a blocked Metropolis Hastings (MH) algorithm using the misspecified independent Poisson likelihood are used on the same 1000 datasets and the results are compared. 500 datasets are simulated using the smaller values of the parameters and 500 datasets using the larger values (see Table 1 in the main text). The only parameters inferred are the transmission parameters  $\beta, \iota$  and  $\pi$  with the severity parameters being fixed at their true, scenario-specific, value.

In the case of **small dependence**, the results show that the posterior distributions obtained with the misspecified independent likelihood are very similar to the ones obtained with the approximated joint likelihood. Figure 1 reports the posterior distributions of the 3 parameters estimated in 5 datasets randomly sampled from the 500 generated datasets. Moreover, Figure 2 displays the distribution of pairwise difference in the variance of the posterior sample:

$$\text{PWD}(\text{Var}(\alpha))^d = \text{Var}(\hat{\alpha}^{\text{JOINT DEP}} | \mathbf{y}^d) - \text{Var}(\hat{\alpha}^{\text{MISS IND}} | \mathbf{y}^d) \quad \alpha = \beta, \pi, \dots; d = 1, 2, \dots, 500$$

and the distribution of pairwise difference in the length of the 95% Credible Interval (CrI) of the posterior sample:

$$\text{PWD}(\text{R}_{95}(\alpha))^d = \text{R}_{95}(\hat{\alpha}^{\text{JOINT DEP}} | \mathbf{y}^d) - \text{R}_{95}(\hat{\alpha}^{\text{MISS IND}} | \mathbf{y}^d) \quad \alpha = \beta, \pi, \dots; d = 1, 2, \dots, 500$$

The figures show an imperceptible difference in the posterior distributions and their precision-summaries between the two models. This is confirmed by quantities such as the proportion of datasets in which the pairwise difference in variance is less than or equal to 0, for each of the parameters reported below. When this quantity is close to 0.5, the variances of the estimates obtained with the two methods are similar within datasets; when this quantity is close to 1 it suggests that the variance of the estimates obtained using the misspecified independent likelihood is systematically larger than the variance of the estimates obtained with the joint likelihood; and when this quantity is close to 0 it highlights that the former variance is systematically smaller than the latter. This results is expected, above all in the case of high dependence scenario, signifying over-precision of the independent-likelihood-driven estimator.

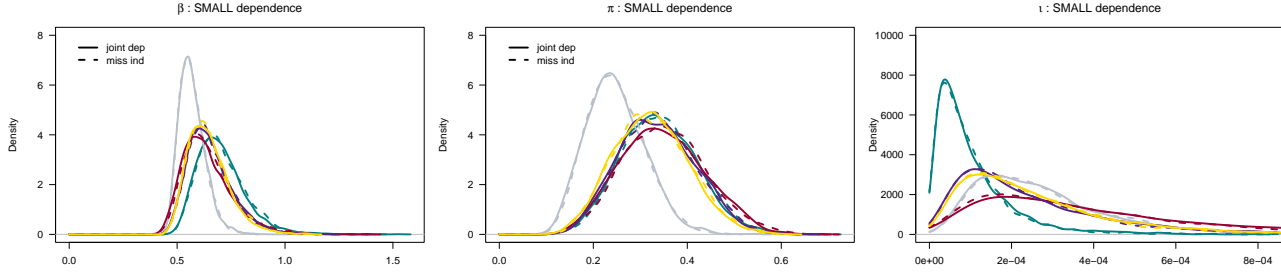

Figure 1: Posterior distribution of the transmission parameters  $\beta$  (left panel),  $\iota$  (centre) and  $\pi$  (right panel) from 5 datasets. The colour of the posterior density identifies the dataset analysed while dashed lines refer to results from the misspecified independent model and filled lines to results from the model approximating the joint dependent likelihood.

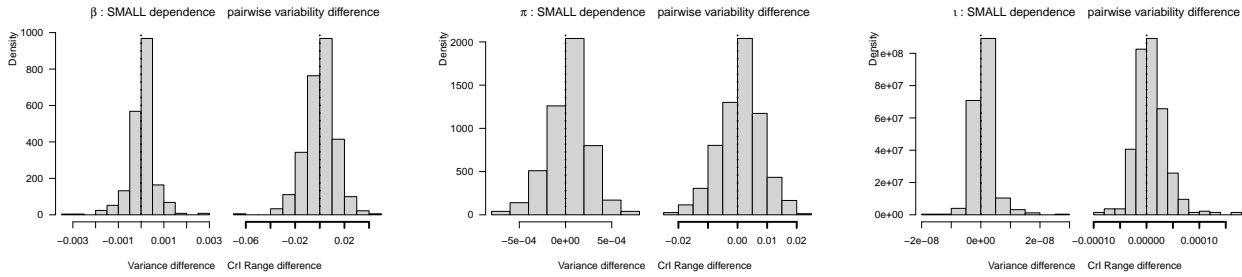

Figure 2: Distribution of the pairwise difference in variance (green plots) and in 95% CrI length (red plots) of the posterior distribution of the transmission parameters  $\beta$  (left panel),  $\iota$  (centre) and  $\pi$  (right panel).

Table 1 reports this quantity for each parameter estimated: here there is no evident signal of systematic difference between methods.

| Parameter | Proportion of $\text{PWD}(\text{Var}) \leq 0$ |
|-----------|-----------------------------------------------|
| $\beta$   | 0.392                                         |
| $\pi$     | 0.390                                         |
| $\iota$   | 0.378                                         |

Table 1: Proportion of datasets in which the pairwise difference of variance is smaller or equal to 0 for the three transmission parameters in the scenario with small dependence.

The same analysis is run on the 500 datasets with a **big dependence** with results reported in Figures 3 and 4.

Here there is a notable difference between the results from the two models: the posterior distributions from the misspecified model that assumes independent data are less variable than the ones derived using the MC approximation of the joint dependent likelihood.

This result was expected since the misspecified model, by assuming independent data, accounts

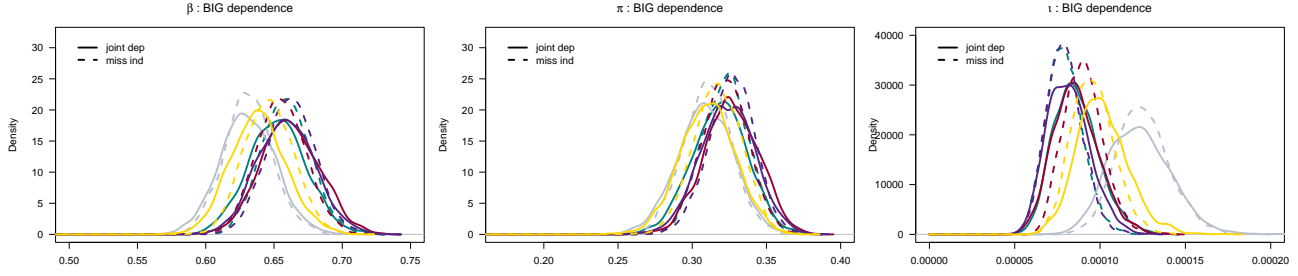

Figure 3: Posterior distribution of the transmission parameters  $\beta$  (left panel),  $\iota$  (centre) and  $\pi$  (right panel) from 5 datasets. The colour of the posterior density identifies the dataset analysed while dashed lines refer to results from the misspecified independent model and filled lines to results from the model approximating the joint dependent likelihood.

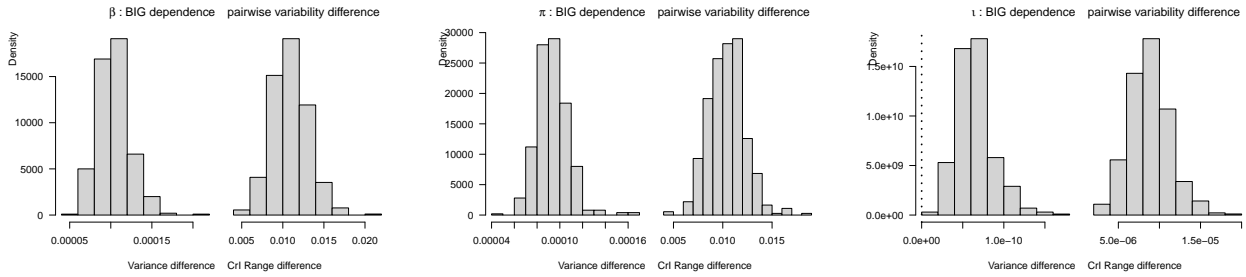

Figure 4: Distribution of the pairwise difference in variance (green plots) and in 95% CrI length (red plots) of the posterior distribution of the transmission parameters  $\beta$  (left panel),  $\iota$  (centre) and  $\pi$  (right panel).

for more information than is inherent in the data. This leads to an overconfidence that can be detected in the underestimation of the posterior variance. Results are confirmed by the proportion of differences less than or equal to 0 for all the parameters (Table 2), strongly suggesting a systematic difference in variability between the two methods. In all the simulated datasets the variance of the posterior distributions of the parameters are smaller in the analysis using the misspecified independent model than in the approximate joint model (Figure 4).

| Parameter | Proportion of $\text{PWD}(\text{Var}) \leq 0$ |
|-----------|-----------------------------------------------|
| $\beta$   | 0                                             |
| $\pi$     | 0                                             |
| $\iota$   | 0                                             |

Table 2: Proportion of datasets in which the pairwise difference of variance is smaller or equal to 0 for the three transmission parameters in the scenario with big dependence.

### 1.2.2 Results for transmission and severity parameters

The same kind of comparison is carried out in a context where inference is drawn both for the transmission and the severity parameters. Here, since more quantities are estimated and due to the high correlation of the parameters of epidemic models, a difference between the results from the two models may be more difficult to spot. Moreover, in this multi-parameter context, convergence is sometimes compromised, particularly in the big-dependence scenario.

The results within a scenario with **small dependence** are reported in Figure 5 and in Figure 6. Neither in the transmission parameters nor in the newly estimated severity parameters, can a large difference be seen.

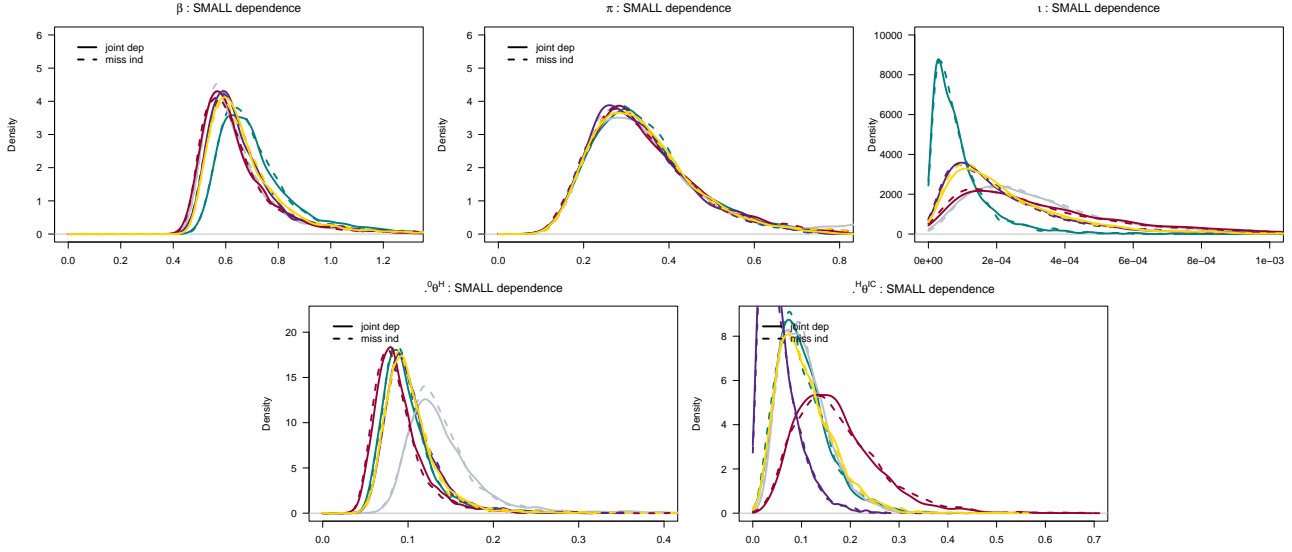

Figure 5: Posterior distribution of the transmission and severity parameters from 5 datasets. The colour of the posterior density identifies the dataset analysed while dashed lines refer to results from the misspecified independent model and filled lines to results from the model approximating the joint dependent likelihood.

The proportions of pairwise differences less than or equal to 0 confirm the non-difference in the variance of the posterior distributions (Table 3).

The same results within a scenario with **big dependence** are plotted in Figures 7 and 8. The only notable difference can be seen in the distribution of  ${}^H\theta^{IC}$ : this parameter is what links the two datasets, since it defines the probability of IC admission conditional on hospitalization. When the two datasets are jointly analysed, they both contribute to the estimation of  ${}^H\theta^{IC}$ , with hospital data informing the Binomial size in Equation ?? and IC data informing the proportion of people in the more-severe state. When the two datasets are considered independently, the hospital data do not play any role in the inference of  ${}^H\theta^{IC}$ .

The proportions of pairwise differences less than or equal to 0 confirm the observations above: the variance of the posterior sample of the parameter  ${}^H\theta^{IC}$  is always lower when inference is drawn with the approximation to the joint dependent likelihood compared to when the misspecified independent model is adopted (Table 4).

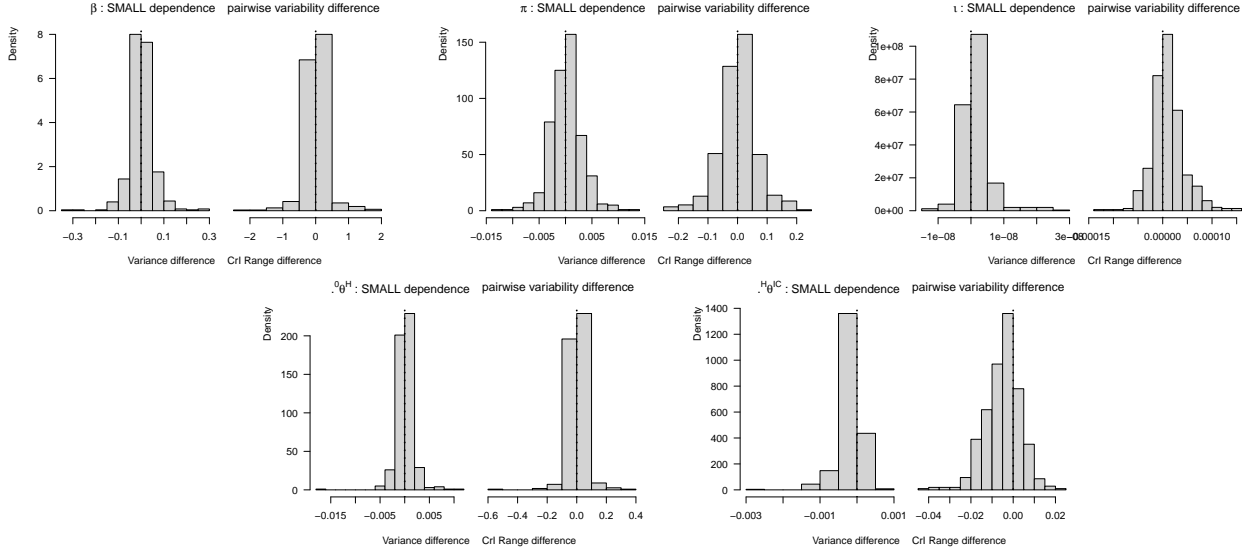

Figure 6: Distribution of the pairwise difference in variance (green plots) and in 95% CrI length (red plots) of the posterior distribution of the transmission and severity parameters.

| Parameter         | Proportion of $\text{PWD}(\text{Var}) \leq 0$ |
|-------------------|-----------------------------------------------|
| $\beta$           | 0.498                                         |
| $\pi$             | 0.464                                         |
| $\iota$           | 0.348                                         |
| ${}^0\theta^H$    | 0.466                                         |
| ${}^H\theta^{IC}$ | 0.778                                         |

Table 3: Proportion of datasets in which the pairwise difference of variance is smaller or equal to 0 for the transmission and severity parameters in the scenario with small dependence.

| Parameter         | Proportion of $\text{PWD}(\text{Var}) \leq 0$ |
|-------------------|-----------------------------------------------|
| $\beta$           | 0.554                                         |
| $\pi$             | 0.546                                         |
| $\iota$           | 0.202                                         |
| ${}^0\theta^H$    | 0.566                                         |
| ${}^H\theta^{IC}$ | 1                                             |

Table 4: Proportion of datasets in which the pairwise difference of variance is smaller or equal to 0 for the transmission and severity parameters in the scenario with big dependence.

The remaining parameters, do not show any significant difference in the variance of their posterior distributions.

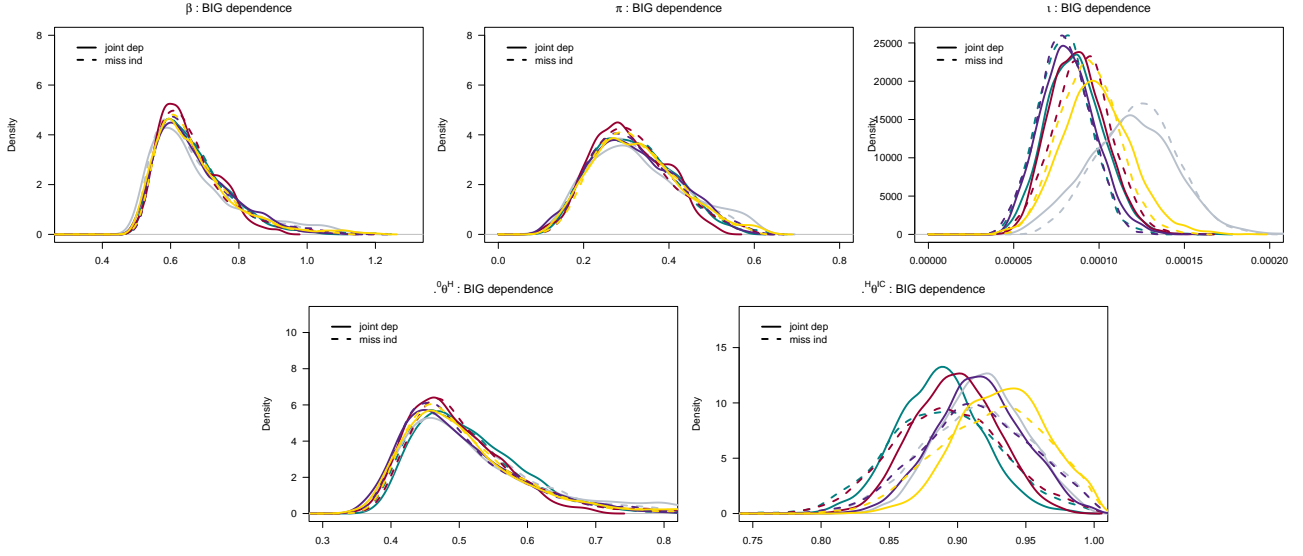

Figure 7: Posterior distribution of the transmission and severity parameters from 5 datasets. The colour of the posterior density identifies the dataset analysed while dashed lines refers to results from the misspecified independent model and filled lines to results from the model approximating the joint dependent likelihood.

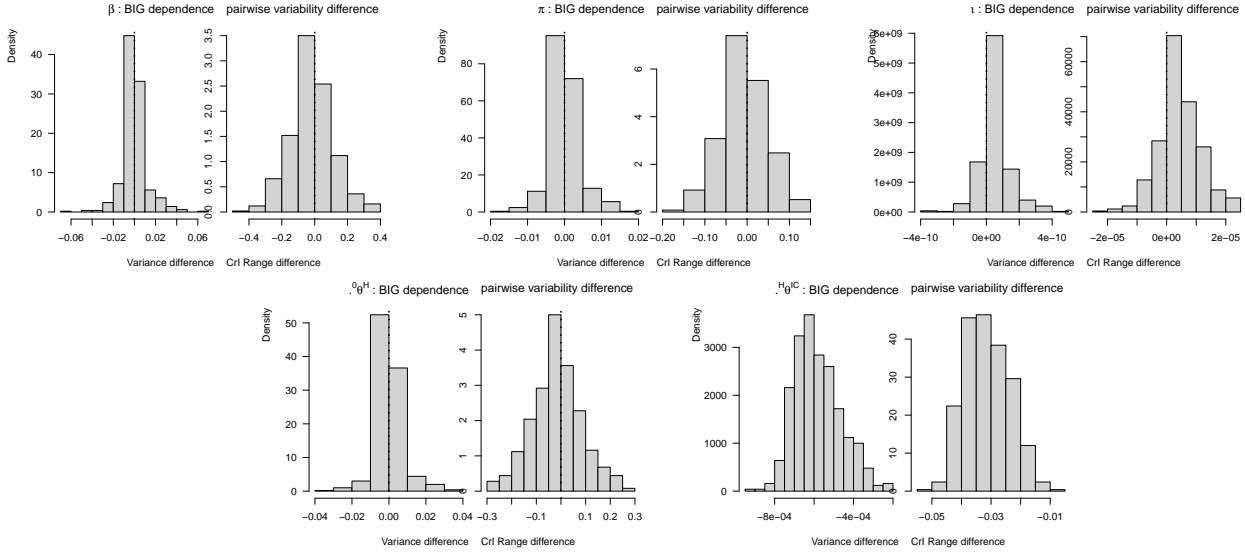

Figure 8: Distribution of the pairwise difference in variance (green plots) and in 95% CrI length (red plots) of the posterior distribution of the transmission and severity parameters from all the datasets.

### 1.2.3 Influential parameters

As a final comparison a further investigation into the main cause of the difference is undertaken. Starting from the small-dependence scenario, one at a time, each parameter of Table 1 of the main text, is allowed to take the larger value in simulating the 500 datasets.

Estimates of the five parameters are then obtained according to the misspecified independent and the joint dependent model. The posterior distributions and the plots of the precision statistics are here omitted. While a detectable difference in the results is observed when all the parameters affecting the level of dependence vary, the same cannot be said when each parameter increases alone. Differences are less evident, with the probability of detection in IC being the most influential parameter, as shown in Table 5, where each column corresponds to a scenario where all the parameters but the header of the column are assumed small.

| Increased Parameter | ${}^0\theta^H$                  | ${}^H\theta^{IC}$ | $\zeta^H$ | $\zeta^{IC}$ |
|---------------------|---------------------------------|-------------------|-----------|--------------|
| Parameter           | Proportion of $PWD(Var) \leq 0$ |                   |           |              |
| $\beta$             | 0.468                           | 0.454             | 0.296     | 0.490        |
| $\pi$               | 0.450                           | 0.454             | 0.214     | 0.496        |
| $\iota$             | 0.342                           | 0.082             | 0.052     | 0.032        |
| ${}^0\theta^H$      | 0.476                           | 0.458             | 0.290     | 0.464        |
| ${}^H\theta^{IC}$   | 0.682                           | 0.940             | 0.072     | 0.994        |

Table 5: Proportion of datasets in which the pairwise difference of variance is smaller or equal to 0 for the transmission and severity parameters in the scenario with small dependence except for the respective column-name parameter.

## 2 Supplement to Section 5

An extensive description of the model, the inferential methods and the results of the analysis of influenza season 2017/18 is reported here.

### 2.1 Model assumption

A full DAG of the model and its parameters is drawn in Figure 9. Its main elements are reported below.

#### 2.1.1 Transmission and first severity layer

Denote by  $\xi_u^0$  the number of new infections generated during day  $u$ . A deterministic *SEIR* transmission model, is assumed so that  $\xi_u^0$  is a function of the parameters  $\pi, \iota, \beta, \sigma, \gamma, \kappa$ , representing the proportion of individuals initially immune; the proportion of initially infected/infectious individuals; the transmission rate; the rate of becoming infectious; the recovery rate; and the school-closure effect, respectively.

The infection processes of individuals who will experience hospital admissions,  ${}^0X^H$ , and influenza-

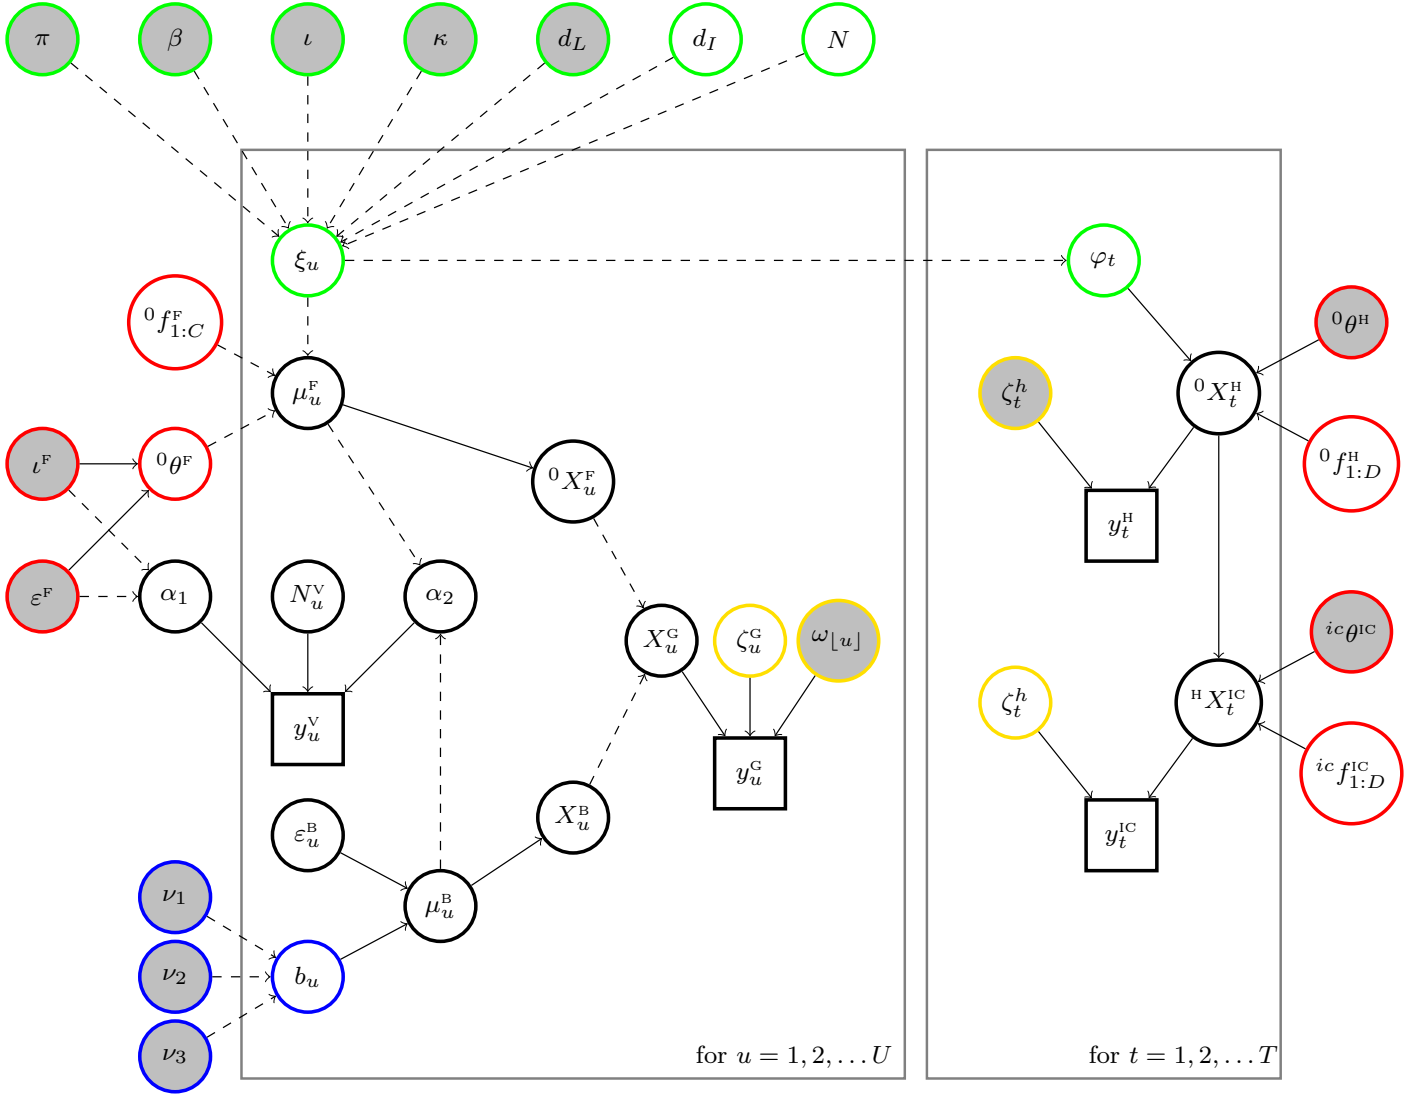

Figure 9: Model DAG The model of GP data ( $y_u^G$ ) and virological data ( $y_u^V$ ) over days ( $u = 1, \dots, U$ ) is illustrated in the left panel; the model for hospital data ( $y_t^H$ ) and IC data ( $y_t^{IC}$ ) over weeks ( $t = 1, \dots, T$ ) is illustrated in the right panel. The observed data are represented by squares, while the r.v.s are represented by circles and they can be either basic parameters (for which we draw inference or assume known), functional parameters (deterministically depending on basic parameters), or r.v.s depending on functional or basic parameters. The filled grey circles are the parameters for which we draw inference. Parameters and hidden quantities have their outer circle coloured according to the process they influence: transmission is green; severity is red; detection is yellow; background ILI is blue; other or more than one process is black. Lastly, stochastic dependence are solid arrows and deterministic dependence are dashed arrows.

related GP consultations,  ${}_u^0 X^F$ , are assumed to follow a time non-homogeneous Poisson process, i.e.:

$$\begin{aligned} \left( {}_u^0 X^H \middle| \xi_u^0, {}^0\theta^H \right) &\sim \text{Pois} \left( {}^0\theta^H \cdot \xi_u^0 \right) & \text{for } u = 0, 1, \dots, U \\ \left( {}_u^0 X^F \middle| \xi_u^0, {}^0\theta^F \right) &\sim \text{Pois} \left( {}^0\theta^F \cdot \xi_u^0 \right) & \text{for } u = 0, 1, \dots, U \end{aligned} \quad (1)$$

with  ${}^0\theta^F$  and  ${}^0\theta^H$  denoting the probability of being visited by a GP and being admitted to hospital, respectively.

### 2.1.2 GP-consultations

Let  ${}^0 f_{0:C}^F = ({}^0 f_0^F, {}^0 f_1^F, \dots, {}^0 f_C^F)$  denote the distribution of  $0, 1, \dots, C$  days occurring between infection and the visit to the GP. The process of daily influenza-related GP consultations, can be shown to be a non-homogeneous Poisson process:

$$\left( X_u^F \middle| {}^0\theta^F, \xi_{1:U}^0, {}^0 f_{0:C}^F \right) \sim \text{Pois} (\mu_u^F) \quad \text{for } u = 0, 1, \dots, U \quad (2)$$

where  $\mu_u^F = {}^0\theta^F \cdot \sum_{c=0}^C \xi_{u-c}^0 \cdot {}^0 f_c^F$ . The variability of the influenza-related GP cases is further affected by the uncertainty on the parameter  ${}^0\theta^F$  encoded by the assumed prior:

$$\left( {}^0\theta^F \middle| \iota^F, \varepsilon^F \right) \sim \text{Gamma}(\iota^F \varepsilon^F, \varepsilon^F). \quad (3)$$

Background, non-influenza cases appear in GP consultation data; these endemic cases of other respiratory viruses and bacterial infections often follow a yearly seasonality, peaking around the same time as the seasonal influenza epidemic (Paul, Held, and Toschke, 2008). Daily background cases are denoted by  $X_u^B$ , are assumed to follow a Poisson distribution with time varying rate  $\mu_u^B$ , distributed according to a Gamma r.v. with mean  $b_u$  and variance  $\frac{1}{\varepsilon^B} = \frac{\sum_{c=0}^C \xi_{u-c}^0 \cdot {}^0 f_c^F}{\varepsilon^F}$ :

$$\begin{aligned} \left( X_u^B \middle| \mu_u^B \right) &\sim \text{Pois} (\mu_u^B) & \text{for } u = 0, 1, \dots, U \\ \left( \mu_u^B \middle| b_u, \varepsilon^B \right) &\sim \text{Gamma}(b_u \varepsilon^B, \varepsilon^B) & \text{for } u = 0, 1, \dots, U. \end{aligned}$$

Here the mean  $b_u$  encapsulates the seasonality pattern by being defined as a weekly-varying sine-cosine oscillation with parameters  $\nu_1, \nu_2$ , and  $\nu_3$ .

The total number of GP consultations,  $X_u^G$ , includes both influenza-related cases,  $X_u^F$ , and endemic background cases,  $X_u^B$ , forming a Poisson process with time-varying rate:

$$\begin{aligned} X_u^G &= X_u^F + X_u^B & \text{for } u = 0, 1, \dots, U \\ \left( X_u^G \middle| \mu_u^F, \mu_u^B \right) &\sim \text{Pois} (\mu_u^F + \mu_u^B) & \text{for } u = 0, 1, \dots, U. \end{aligned} \quad (4)$$

The probability of detecting an ILI case, conditionally on visiting the GP, is proportional to the day-specific catchment population of the practices participating in the collection scheme on day  $u$ , here denoted by  $\zeta_u^G$ .

Further, the probability of attending a GP practice is subject to weekly fluctuations, caused by the weekend closure of GP practices, which is included as a day-of the week effect  $\omega_{[u]}$ , for  $[u] \in \{1=\text{Mon}, 2=\text{Tue}, 3=\text{Wed}, 4=\text{Thu}, 5=\text{Fri}, 6=\text{Sat}, 7=\text{Sun}\}$ . Interpreting  $\omega_{[u]}$  as a distortion factor, for identifiability reason, it is useful to assume that its geometric mean over the 7 days is equal to 1, so that the rate of GP consultation is only re-distributed over the 7 week days according to the opening time of the GP practices, leading to:

$$\prod_{i \in \{1,2,3,4,5,6,7\}} \omega_i = 1$$

The reported number of GP consultations for ILI at time  $u$ ,  $Y_u^G$  is therefore :

$$\left( Y_u^G \middle| x_u^G, \zeta_u^G, \omega_{[u]} \right) \sim \text{Bin} \left( x_u^G; \zeta_u^G \omega_{[u]} \right) \quad \text{for } u = 0, 1, \dots, U \quad (5)$$

Given the distributional assumptions of Equations 2, 3, 4, and 5, the GP ILI data can be shown to be distributed as a Negative Binomial r.v.:

$$\left( Y_u^G \middle| \xi_{1:U}^0, {}^0f_{0:C}^F, \zeta_u^G, \omega_{[u]}, \iota^F, \varepsilon^F, g_u, \varepsilon^B \right) \sim \text{NB} \left( \varepsilon^F \iota^F + \frac{b_u \varepsilon^F}{\sum_{c=0}^C \xi_{u-c}^0 {}^0f_c^F}; 1 + \frac{\zeta_u^G \omega_{[u]} \sum_{c=0}^C \xi_{u-c}^0 {}^0f_c^F}{\varepsilon^F} \right)$$

for  $u = 0, 1, \dots, U$ .

The virology data enable to uncover the proportion of ILI cases genuinely affected by the influenza virus. The number of positive tests at each day  $u$ ,  $Y_u^V$ , is assumed to be a Binomial sample from the number of tests taken  $N_u^V$  with probability  $\frac{\mu_u^F}{\mu_u^F + \mu_u^B}$ :

$$\left( Y_u^V \middle| N_u^V, \mu_u^F, \mu_u^B \right) \sim \text{Binom} \left( N_u^V; \frac{\mu_u^F}{\mu_u^F + \mu_u^B} \right) \quad \text{for } u = 0, 1, \dots, U$$

Following from the distributional assumptions above,  $\mu_u^F$  and  $\mu_u^B$  are assumed to be Gamma distributed with the same rate parameter;; this implies that the quantity  $\frac{\mu_u^F}{\mu_u^F + \mu_u^B}$  is distributed as a Beta r.v.,

$$\left( \frac{\mu_u^F}{\mu_u^F + \mu_u^B} \middle| b_u, \xi_{1:U}^0, {}^0f_{0:C}^F, \iota^F, \varepsilon^F \right) \sim \text{Beta} \left( \iota^F \varepsilon^F, b_u \frac{\varepsilon^F}{\sum_{c=0}^C \xi_{u-c}^0 {}^0f_c^F} \right) \quad \text{for } u = 0, 1, \dots, U$$

resulting in the data  $Y_u^V$  being distributed according to the Beta-Binomial below:

$$\left( Y_u^V \middle| N_u^V, b_u, \xi_{1:U}^0, {}^0f_{0:C}^F, \iota^F, \varepsilon^F \right) \sim \text{BetaBin} \left( N_u^V; \alpha_1 = \iota^F \varepsilon^F; \alpha_2 = b_u \frac{\varepsilon^F}{\sum_{c=0}^C \xi_{u-c}^0 {}^0f_c^F} \right) \quad (6)$$

for  $u = 0, 1, \dots, U$ .

### 2.1.3 Hospitalization and IC admissions

A model for dependent data on hospitalizations and IC-admissions data is illustrated in Section ?? . Here too the joint likelihood is factorised in the marginal distribution of the IC admissions  $Y_{1:T}^{\text{IC}}$ , from the Poisson distribution of Equation ?? , and the distribution of the hospitalizations  $Y_{1:T}^{\text{H}}$  conditionally on IC data approximated via MC integration as proposed in Algorithm 2.

A model for the hospitalizations and IC-admissions data is proposed in Section 3 of the main text, with the two data streams analysed jointly, since they are intrinsically dependent. Denote by  $\varphi_t^0$  number of new infections generated at week  $t$  from the beginning of the epidemic, resulting from a deterministic transformation of the daily infections:  $\varphi_t^0 = \sum_{u=7t-6}^{7t} \xi_u^0$ . Denote by  ${}^{\text{H}}\theta^{\text{IC}}$  the probability of IC admission given hospitalization; by  ${}^0f_d^{\text{H}}$  and  ${}^{\text{H}}f_d^{\text{IC}}$  the discrete probability of  $d$  weeks elapsing between infection and hospitalization and hospitalization and IC admission, respectively; by  $\zeta_t^{\text{H}}$  and  $\zeta_t^{\text{IC}}$  the probability of being detected in hospital and in IC, respectively.

The data-generating process can be expressed as a series of Binomial and Multinomial steps from the initial Poisson process of the infections that will be hospitalised,  ${}^0X^{\text{H}}$ .

$$\begin{aligned} \left( {}^0X_{t:t+D}^{\text{H}} \middle| {}^0x^{\text{H}}, {}^0f_{0:D}^{\text{H}} \right) &\sim \text{Multi}({}^0x^{\text{H}}, {}^0f_{0:D}^{\text{H}}) \quad , \quad X_t^{\text{H}} = \sum_{d=0}^D t-d {}^0X_d^{\text{H}} \\ \left( {}^{\text{H}}X_t^{\text{IC}} \middle| x_t^{\text{H}}, {}^{\text{H}}\theta^{\text{IC}} \right) &\sim \text{Bin}(x_t^{\text{H}}, {}^{\text{H}}\theta^{\text{IC}}) \\ \left( {}^{\text{H}}X_{t:t+D}^{\text{IC}} \middle| {}^{\text{H}}x^{\text{IC}}, {}^{\text{H}}f_{0:D}^{\text{IC}} \right) &\sim \text{Multi}({}^{\text{H}}x^{\text{IC}}, {}^{\text{H}}f_{0:D}^{\text{IC}}) \quad , \quad X_t^{\text{IC}} = \sum_{d=0}^D t-d {}^{\text{H}}X_d^{\text{IC}} \\ \left( Y_t^{\text{H}} \middle| x_t^{\text{H}}, \zeta_t^{\text{H}} \right) &\sim \text{Bin}(x_t^{\text{H}}, \zeta_t^{\text{H}}) \\ \left( Y_t^{\text{IC}} \middle| x_t^{\text{IC}}, \zeta_t^{\text{IC}} \right) &\sim \text{Bin}(x_t^{\text{IC}}, \zeta_t^{\text{IC}}) \end{aligned}$$

for time  $t = 1, \dots, T$ . This model leads to the two marginal data distributions:

$$\begin{aligned} \left( Y_t^{\text{H}} \middle| \zeta_t^{\text{H}}, {}^0\theta^{\text{H}}, \xi_{0:T}^0, {}^0f_{0:D}^{\text{H}} \right) &\sim \text{Pois} \left( \zeta_t^{\text{H}} \cdot {}^0\theta^{\text{H}} \cdot \sum_{d=0}^D \varphi_{t-d}^0 \cdot {}^0f_d^{\text{H}} \right) \\ \left( Y_t^{\text{IC}} \middle| \zeta_t^{\text{H}}, {}^0\theta^{\text{H}}, \xi_{0:T}^0, {}^0f_{0:D}^{\text{H}}, {}^{\text{H}}\theta^{\text{IC}}, {}^0f_{0:D}^{\text{IC}} \right) &\sim \text{Pois} \left( \zeta_t^{\text{IC}} \cdot {}^{\text{H}}\theta^{\text{IC}} \cdot {}^0\theta^{\text{H}} \cdot \sum_{d=0}^D \sum_{g=0}^d \varphi_{t-d-g}^0 \cdot {}^0f_d^{\text{H}} \cdot {}^{\text{H}}f_g^{\text{IC}} \right) \end{aligned}$$

To compute the joint distribution of  $(Y_t^{\text{H}}; Y_t^{\text{IC}})$  for  $t = 1, \dots, T$ , a simulation-based algorithm is adopted: the marginal distribution of the IC admissions  $Y_{1:T}^{\text{IC}}$  is computed from the Poisson distribution above and the distribution of the hospitalizations  $Y_{1:T}^{\text{H}}$  conditionally on IC data is approximated via MC integration as illustrated in Section 1.1. above.

## 2.2 Prior distributions

The prior distributions on the parameters involved in the model are described below and further summarised in Table 6 (last column).

In the transmission model, uniform priors are assumed for the transmission rate,  $\beta$ , and the initial proportion of exposed/infectious individuals,  $\iota$ . The initial proportion of immune people,  $\pi$ , is assumed to be distributed as a Beta r.v. centred in 0.375; this result was obtained from the analysis of serological data at the end of the previous season by collaborators at Public Health England (PHE) Charlett, 2018. The average latent period is assumed to be Log-Normally distributed with mean 2 days and the average infectious period is assumed known and equal to 3.14 days; these two values are taken from Birrell et al., 2011. The holidays factor,  $\kappa$ , models the increase or decrease in infection rate during school closure as follows:

$$S_{t+1} = S_t - (1 + \kappa) \cdot \beta \delta S_t \frac{I_t}{N} \quad \text{for } t \in \text{school holidays}$$

$\kappa$  can take any value between -1 and  $+\infty$ , with negative values indicating a decrease of infectiousness during school holidays and positive values indicating an increase of infectiousness during school closure. This parameter is assigned a shifted Log-Normal prior distribution centred on 0. Lastly, the population size, is fixed to the latest available data from the Office of National Statistics (ONS),  $N = 55268100$ , i.e. the mid-2016 estimates Office of National Statistics, 2017.

The main severity parameters are  ${}^0\theta^F$ ,  ${}^0\theta^H$  and  ${}^H\theta^{IC}$ . The probability of flu-related GP consultations,  ${}^0\theta^F$ , has hyper-parameters  $\iota^F$  and  $\varepsilon^F$ . The former is given a Uniform prior between 0 and 1 and the precision  $\varepsilon^F$  is given a Uniform prior between 0 and 5000. Sampling directly from the priors leads to a Uniform-like distribution between 0 and 1 for  ${}^0\theta^F$ .  ${}^0\theta^H$  and  ${}^H\theta^{IC}$  are both given Uniform priors between 0 and 1.

The discrete waiting-times between consecutive severe events are assumed known. The distribution of the time from infection to flu-related GP consultation,  ${}^0f_{0:C}^F$ , is obtained by discretising in days the density of a Gamma (3.41, 0.83) (taken from the sum of the prior distributions assumed in Birrell et al., 2011). The distribution of the time from infection to hospitalization,  ${}^0f_{0:D}^H$ , and from hospitalization to IC admission,  ${}^Hf_{0:D}^{IC}$ , are obtained by discretising in days two Exponential distributions with rate 0.32 and 0.4, respectively (from the analysis of individual data from the USSS sentinel scheme).

The mean of the background ILI consultations is centred on a sine-cosine transformation of the weeks. The parameters  $\nu_1, \nu_2$  and  $\nu_3$  specifying this behaviour are assigned an informative prior obtained from fitting an *HHH model* Held, Höhle, and Hofmann, 2005 to GP data from January 2015 to September 2017.

Six parameters for the day of the week effect are to be estimated ( $\omega_4$ , the effect of Thursday). The parameter vector  $(\omega_1, \omega_2, \omega_3, \omega_5, \omega_6, \omega_7)$  is assigned multivariate Log-Normal prior centred in 1, implicitly assuming no effect of the day of the week, and every  $\text{xlog}(\omega)$  is given variance equal to 0.4.

$$\begin{pmatrix} \omega_1 \\ \omega_2 \\ \omega_3 \\ \omega_5 \\ \omega_6 \\ \omega_7 \end{pmatrix} \sim \text{Log-Normal}(\log(1), V_\omega)$$

$V_\omega$  is formulated so that the equality of variances is preserved also for the parameter  $\omega_4 =$

$1 / \prod_{i \in \{1,2,3,5,6,7\}} \omega_i$ . The derivation from Birrell et al., 2016, leads to:

$$V_\omega = 0.16 \begin{pmatrix} 1 & -1/6 & -1/6 & -1/6 & -1/6 & -1/6 \\ -1/6 & 1 & -1/6 & -1/6 & -1/6 & -1/6 \\ -1/6 & -1/6 & 1 & -1/6 & -1/6 & -1/6 \\ -1/6 & -1/6 & -1/6 & 1 & -1/6 & -1/6 \\ -1/6 & -1/6 & -1/6 & -1/6 & 1 & -1/6 \\ -1/6 & -1/6 & -1/6 & -1/6 & -1/6 & 1 \end{pmatrix}$$

The detection parameters are mainly informed by the catchment population of the reporting trusts or GP clinics, as a proportion of the population of England, denoted by  $d_u^G$  for GP data,  $d_t^H$  for hospital data and  $d_t^{IC}$  for IC data. Specifically:  $\zeta_u^G = d_u^G$  and  $\zeta_t^{IC} = d_t^{IC}$ , while  $\zeta_t^H$ , as mentioned above, is given a Beta prior with hyper-parameters  $d_t^H$ , fixed, and  $\epsilon^H$ , influencing the precision of the data, being assigned a uniform prior between 0 and 100.

| Parameter                                                      | Name               | Posterior Me (95%CrI)                   | Prior                                        |
|----------------------------------------------------------------|--------------------|-----------------------------------------|----------------------------------------------|
| Transmission rate                                              | $\beta$            | 0.6189 (0.5284-0.747)                   | Uniform(0,4)                                 |
| Initial immunity                                               | $\pi$              | 0.3744 (0.2836-0.4709)                  | Beta(37.5,62.5)                              |
| Initial exposed/infectious                                     | $\iota$            | (1.519 (0.71756-2.668)) $\cdot 10^{-4}$ | Uniform(0, 0.1)                              |
| Average latent period                                          | $d_L = 2/\sigma$   | 3.5437 (1.3458-6.2044)                  | Log-Normal(log(2),0.5)                       |
| Average infectious period                                      | $d_I = 2/\gamma$   | -                                       | PP at 3.14                                   |
| Total population                                               | N                  | -                                       | PP at 55268100                               |
| Factor for holidays                                            | $\kappa$           | 0.4273 (0.2523-0.6311)                  | shifted Log-Normal(0,1)                      |
| Mean of case to GP risk                                        | $\iota^F$          | 0.0025 (0.0018-0.0038)                  | Uniform(0,1)                                 |
| Precision of case to GP risk                                   | $\epsilon^F$       | 544.5252 (350.1071-804.3077)            | Uniform(0,5000)                              |
| Case to hospitalization risk                                   | ${}^0\theta^H$     | 0.0032 (0.0022-0.0049)                  | Uniform(0,1)                                 |
| Hospital to IC risk                                            | ${}^H\theta^{IC}$  | 0.0667 (0.0574-0.078)                   | Uniform(0,1)                                 |
| Time infection $\rightarrow$ GP visit                          | ${}^0f_{0:C}^F$    | -                                       | PP Gamma (3.41,0.83)                         |
| Time infection $\rightarrow$ hospitalization                   | ${}^0f_{0:C}^H$    | -                                       | PP Exp (0.32)                                |
| Time hospitalization $\rightarrow$ IC                          | ${}^Hf_{0:C}^{IC}$ | -                                       | PP Exp (0.4)                                 |
| background par 1                                               | $\nu_1$            | 6.7618 (6.6705-6.8495)                  | Norm(4.66, 0.17)                             |
| background par 2 (sin)                                         | $\nu_2$            | -0.008 (-0.0987-0.0792)                 | Norm(-0.2, 0.11)                             |
| background par 3 (cos)                                         | $\nu_3$            | 0.7789 (0.6742-0.8862)                  | Norm( 0.99, 0.08)                            |
| Monday, Tuesday, Wednesday,<br>Friday, Saturday, Sunday effect | $\omega_1$         | 4.067(3.6789 – 4.5025)                  | Log-Normal(log(1), $V_\omega$ )              |
|                                                                | $\omega_2$         | 3.0727(2.7635 – 3.4208)                 |                                              |
|                                                                | $\omega_3$         | 2.9227(2.6261 – 3.2603)                 |                                              |
|                                                                | $\omega_5$         | 2.9043(2.5997 – 3.2598)                 |                                              |
|                                                                | $\omega_6$         | 0.0939(0.0781 – 0.1122)                 |                                              |
|                                                                | $\omega_7$         | 0.0375(0.0291 – 0.0479)                 |                                              |
| Thursday effect                                                | $\omega_4$         | -                                       | $1 / \prod_{i \in \{1,2,3,5,6,7\}} \omega_i$ |

Table 6: Posterior summaries and Prior distributions of all the parameters of the model.  
PP stands for *Point Prior*.

## 2.3 Inference

The goal of the inference is to obtain posterior draws from the unknown parameter vector

$$\boldsymbol{\theta} = (\beta, \pi, \iota, d_L, \kappa, \iota^F, \varepsilon^F, {}^0\theta^H, {}^h\theta^{IC}, \nu_1, \nu_2, \nu_3, \omega_1, \omega_2, \omega_3, \omega_5, \omega_6, \omega_7).$$

All the elements of  $\boldsymbol{\theta}$  are transformed to lie in  $(-\infty, +\infty)$ , and a bespoke MH sampler is coded to carry out the analysis. The analysis is composed of two phases: firstly a component-wise MH algorithm samples each element of the vector  $\boldsymbol{\theta}$  conditional on the others and in the second block-update phase the whole parameter vector  $\boldsymbol{\theta}$  is sampled jointly. In the component-wise sampling, a Normal random walk is run on the transformed parameter space of  $\boldsymbol{\theta}$ ; the proposal Normal distributions have parameter-specific standard deviations  $s_\beta, s_\pi, s_\iota$ , and so on.

The first phase comprises: 10,000 adaptation iterations, where the values  $s_\beta, s_\pi, s_\iota, \dots, s_{\varepsilon^F}$  are adapted to lead to a desirable acceptance rate (between 0.2 and 0.3); 50,000 burn-in iterations, discarded; and 100,000 sampling iterations, saved with a thinning factor of 500. Three parallel chains are run, resulting in 6,000 samples for each parameter.

The samples are used to estimate  $\mathcal{S}$ , the variance-covariance matrix for the 19-variate Normal proposal for the second block-update phase: the observed variance-covariance matrix of the sample is multiplied by a factor which is adapted for the first 100,000 iterations of the block-update algorithm; 100,000 iterations are then discarded as burn-in; 1,000,000 iterations are sampled with a thinning factor of 200. Three parallel chains are run, resulting in 15,000 samples for each parameter. MH algorithms are here coupled with MC likelihood estimates for the dependent data, in the fashion of a GIMH Andrieu and Roberts, 2009.

The MH algorithm was coded in R R Core Team, 2018. However the most computationally expensive step is the evaluation of the joint likelihood of the hospital and IC data, for which the Rcpp Eddelbuettel and François, 2010 package is used. The whole analysis ran on a low-performance laptop due to confidentiality constraints given by the data provider, taking in total twenty days.

## 2.4 Results

In what follows, unless specified otherwise, prior distributions are represented in red and posterior distributions are represented in green. Summary statistics of the posterior distributions are reported in Table 6.

### 2.4.1 Transmission

Figure 10 reports the prior-to-posterior plots of the five parameters of the transmission model. Some parameters are highly (or uniquely) informed by the prior distributions. This is the case for the initial immunity  $\pi$ , for which the posterior distribution coincides with its prior, and the average latent period, that is also highly influenced by its prior. Data are characterised by a sudden increase in cases at the end of December and by a prolonged influenza-peak activity. These characteristics result in a shift of  $d_L$  towards higher values, which leads to a longer epidemic, and by posterior values for  $\kappa$ , the school holiday factor, higher than one, allowing transmission to increase during the Christmas break.

The basic and effective reproduction numbers,  $R_0$  and  $R_e(0)$ , are useful summaries of the transmission intensity over the season. Their prior-to-posterior plots are reported in Figure 11, both during school periods and school holidays. During school holidays, transmission becomes more intense, but also more variable, given the uncertainty around the parameter  $\kappa$ .

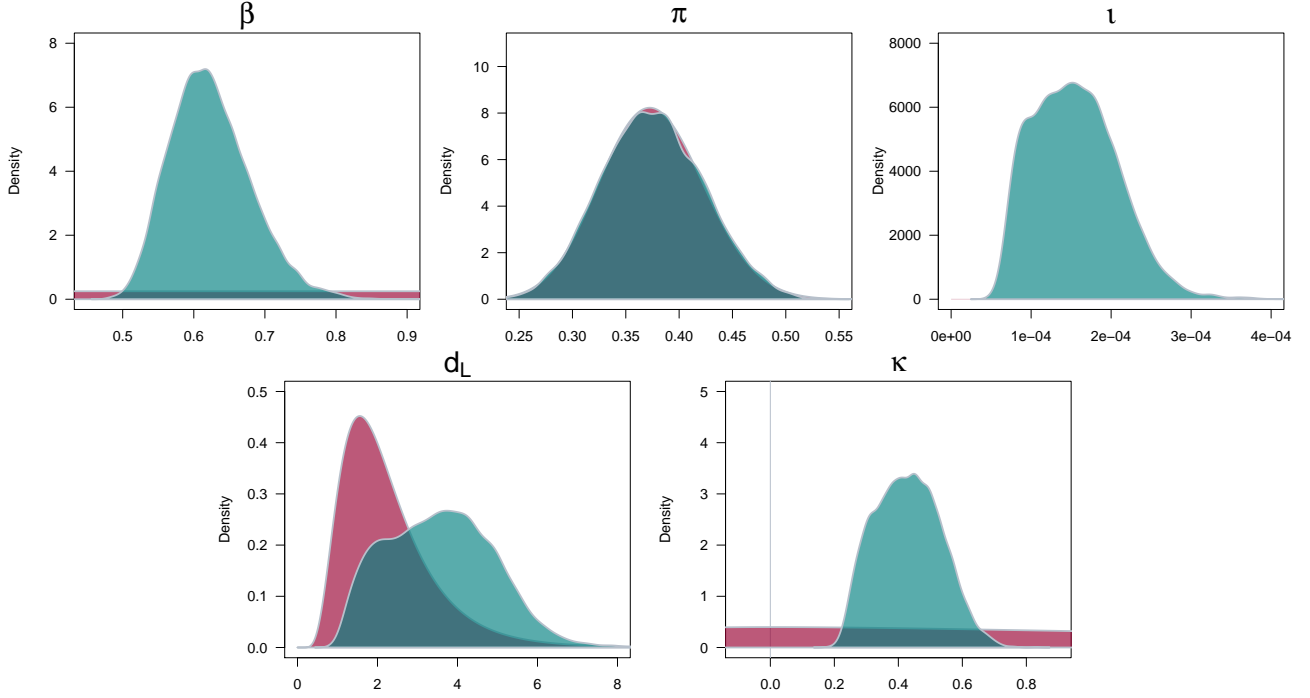

Figure 10: Prior (red) and posterior (green) distributions of the transmission parameters: the transmission rate  $\beta$ , the initial immunity  $\pi$ , the initial proportion of exposed/infectious  $\iota$ , the average latent period  $d_L$ , the factor for school holidays  $\kappa$ .

Finally, to have an overall picture of transmission over the course of the epidemic, the 95% CrIs for the daily number of new infections are plotted in Figure 12. The trajectories clearly show the breakpoints in transmission.

#### 2.4.2 Severity

The severity parameters include:  $\iota^F$  and  $\varepsilon^F$ , i.e. the mean and the precision of the probability of GP consultation given infection,  ${}^0\theta^F$ ; the probability of hospitalization given infection,  ${}^0\theta^H$ ; and the probability of IC admissions given hospitalization,  ${}^H\theta^{IC}$ .

The interpretation of the magnitude of  ${}^0\theta^F$  (and the related  $\iota^F$  and  $\varepsilon^F$ ) necessitates some caution because GP visits are also affected by the day-of-the-week effect. As shown below in the results on the day-of-the-week effect, the risk of GP visit can become four times bigger or 20 times smaller according to the day of the week at which the visit takes place.

The prior-to-posterior plots of the parameters describing severity are reported in Figure 13. All the parameters are highly informed by the data and the posterior distributions give a clear picture of the severity during the 2017/18 influenza epidemic. The probability of hospitalization given infection is around 0.3% and the probability of IC admission given hospitalization stretches between 6 and 7%.

To interpret the results on  $\iota^F$  and  $\varepsilon^F$ , it is useful to draw the distribution of  ${}^0\theta^F$  under the prior

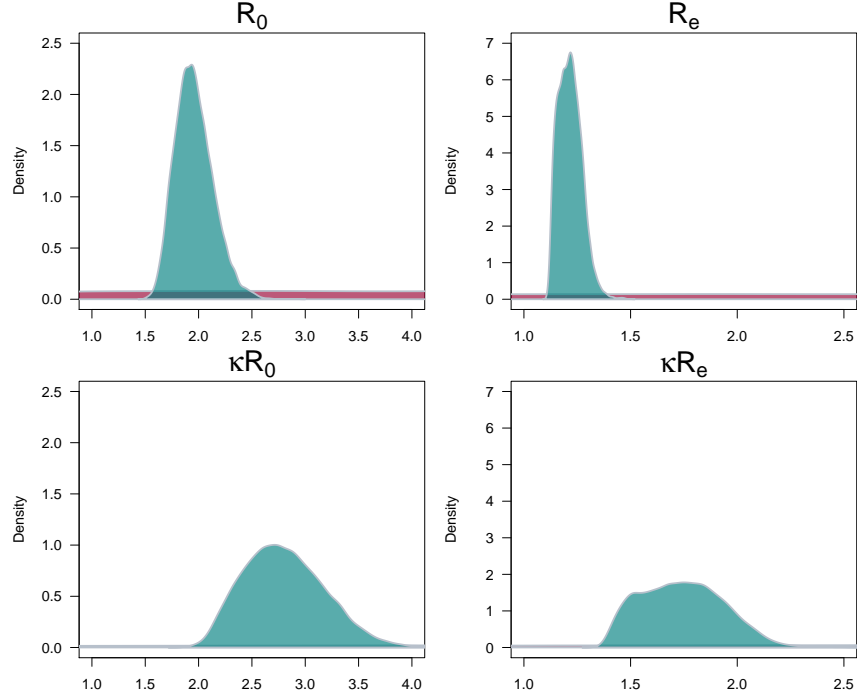

Figure 11: Prior (red) and posterior (green) distribution of the basic and effective reproduction number during school periods (top panels) and during holiday periods (bottom panels).

and posterior distributions of these two parameters. Figure 14 shows that the prior knowledge on  $\theta^F$  was null compared to a well-informed posterior distribution.

### 2.4.3 Background ILI

The prior-to-posterior plots of the three parameters describing the background, non-flu-infected, ILI GP visits are reported in Figure 15.

The resulting average of the background-ILI GP visit process is drawn in Figure 16. Comparing the posterior distribution with the prior, the incidence is slightly delayed but has similar magnitude.

### 2.4.4 Day-of-the-week effect

The prior-to-posterior plots of the day-of-the-week parameters are reported in Figure 17. Monday is the day with highest consultation rate (4 times bigger than the weekly average), while Sunday has the smallest rate (20 times smaller than the average).

The posterior distributions of these parameters, together with the distribution plotted in Figure 14, allow to compute the day-specific risk of GP consultation for influenza cases, plotted in Figure 18.

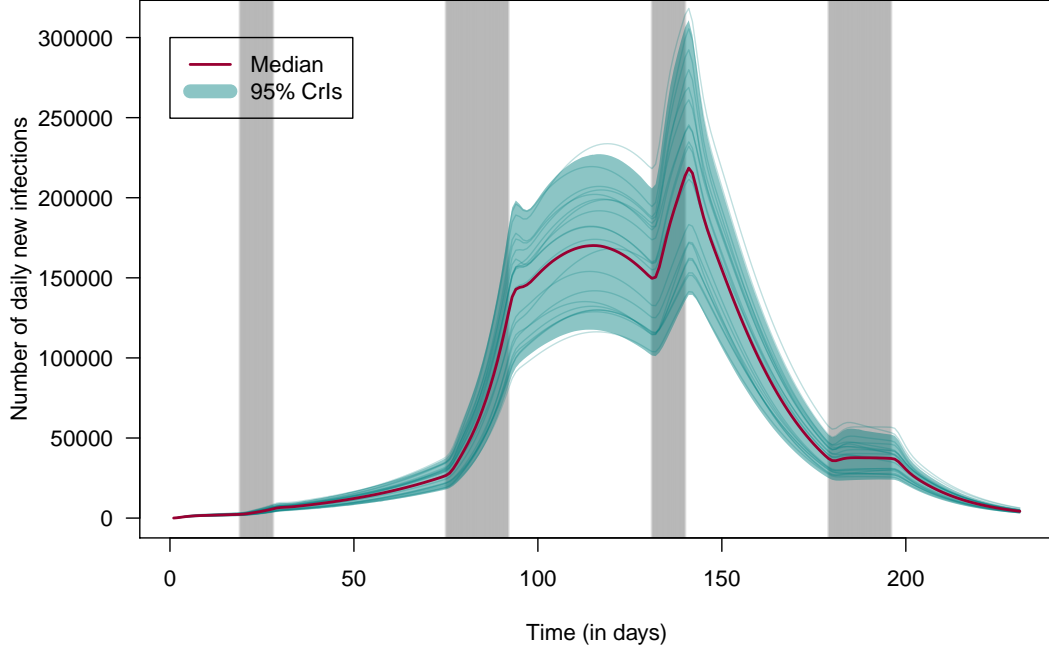

Figure 12: Median (red) and 95% CrIs (green) for the daily number of new infections. The grey areas represent the days corresponding to school holidays. 20 randomly selected trajectories are also computed and plotted as thin green lines.

#### 2.4.5 Reporting

The posterior distribution of the shape parameter of the hospitalization detection is reported in Figure 19. The consequent posterior predictive distribution of the detection parameter  $\zeta_{1:T}^H$  is reported in Figure 20, where the high variability of this parameter can be seen.

#### 2.4.6 Goodness of fit

The goodness of fit of the model is evaluated graphically. Figure 21 plots the predictive posterior distribution of the observed GP consultations for ILI versus the data both on the natural and on the logarithmic scale.

The model describes well the epidemic during its beginning and its end, however the peak of the data is not well reproduced. The variability of the predictions is particularly high in the middle of the epidemic, reflecting the high variability assumed in the severity model and the uncertainty that characterizes the prior distributions of many parameters. The day of the week effect, instead, reflects well the shifts of the observations during weekends, compared to weekdays.

Virology data are much better modelled (Figure 22): the peak of the epidemic is reproduced well and the median predicted number of positives always lies close to the observed data.

Hospital and IC data are to be considered together. While the model proposed above accounts for extra sources of variability for the hospital data (with the Beta prior distribution), the IC data are

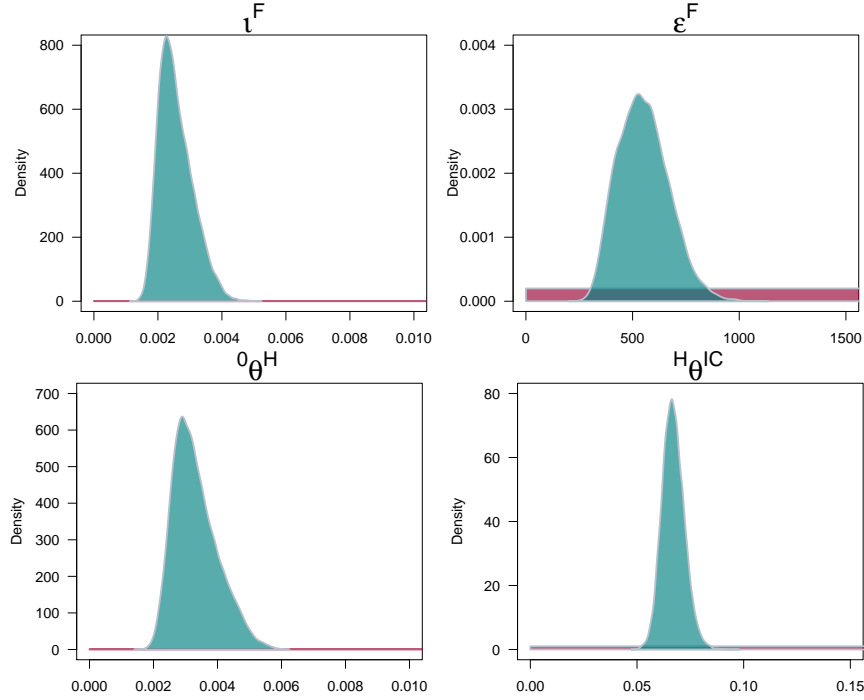

Figure 13: Prior (red) and posterior (green) distributions of the severity parameters:  $\iota^F$ , the mean of the case-GP-consultation risk  ${}^0\theta^F$ ; its precision  $\varepsilon^F$ ; the case hospitalization risk  ${}^0\theta^H$ ; and the probability of IC admission given hospitalization  ${}^H\theta^{IC}$ .

assumed affected by Poisson noise only. Dropping this assumption will compromise the possibility of direct sampling of the hidden states in Algorithm 1. However, over-dispersion parameters have often been found useful, if not essential, to the modelling of infectious-disease data (Bretó et al., 2009). As a result, the IC data are not reproduced well by the model (see Figure 24).

By contrast, the predictive distributions of the hospital data are more variable and the CrIs always include the observed value. Moreover, the median trajectory shows a second peak in correspondence with the observed second peak in the data.

## References

- Andrieu, C. and G. O. Roberts (2009). “The pseudo-marginal approach for efficient Monte Carlo computations”. In: *The Annals of Statistics* 37.2, pp. 697–725.
- Birrell, P. J., G. Ketsetzis, N. J. Gay, B. S. Cooper, A. M. Presanis, R. J. Harris, A. Charlett, X.-S. Zhang, P. J. White, R. G. Pebody, et al. (2011). “Bayesian modeling to unmask and predict influenza A/H1N1pdm dynamics in London”. In: *Proceedings of the National Academy of Sciences* 108.45, pp. 18238–18243.

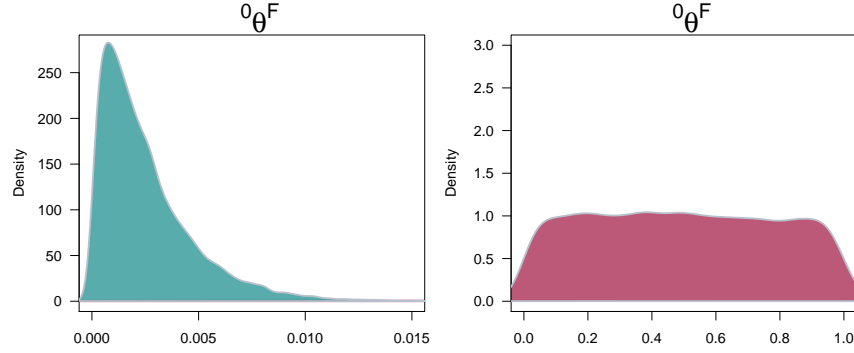

Figure 14: Distribution of  $\theta^F$  under the posterior (left) and prior (right) distribution of the parameters  $\iota^F$  and  $\varepsilon^F$

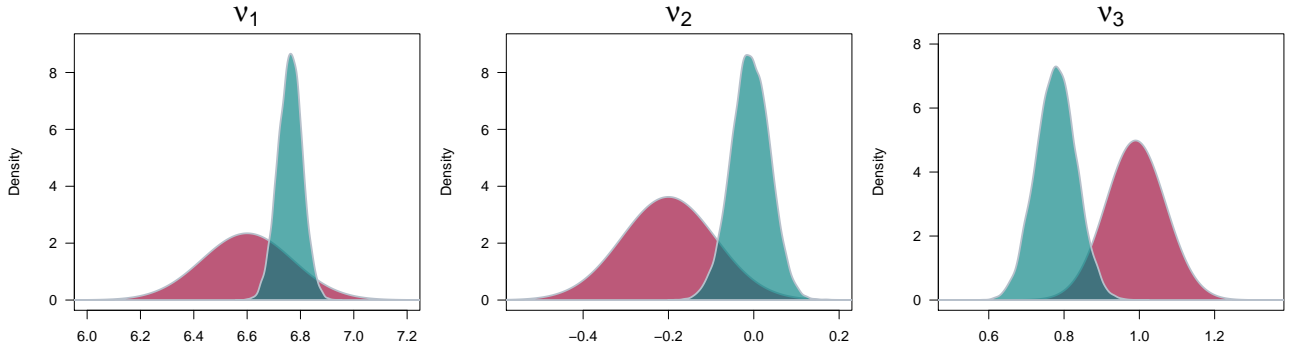

Figure 15: Prior (red) and posterior (green) distributions of the three parameters of the HHH model.

- Birrell, P. J., X.-S. Zhang, R. G. Pebody, N. J. Gay, and D. De Angelis (2016). “Reconstructing a spatially heterogeneous epidemic: Characterising the geographic spread of 2009 A/H1N1pdm infection in England”. In: *Scientific reports* 6.1, pp. 1–10.
- Bretó, C., D. He, E. L. Ionides, and A. A. King (2009). “Time series analysis via mechanistic models”. In: *The Annals of Applied Statistics*, pp. 319–348.
- Brooks, S., A. Gelman, G. Jones, and X.-L. Meng (2011). *Handbook of markov chain monte carlo*. CRC press.
- Charlett, A. (2018). “Personal communication on the level of immunity priori 2017/18 Influenza season”. PHE.
- Eddelbuettel, D. and R. François (2010). “Rcpp syntactic sugar”. In.
- Held, L., M. Höhle, and M. Hofmann (2005). “A statistical framework for the analysis of multivariate infectious disease surveillance counts”. In: *Statistical modelling* 5.3, pp. 187–199.
- Office of National Statistics (2017). “Population Estimates for UK, England and Wales, Scotland and Northern Ireland, mid 2016”. In.
- Paul, M., L. Held, and A. M. Toschke (2008). “Multivariate modelling of infectious disease surveillance data”. In: *Statistics in medicine* 27.29, pp. 6250–6267.

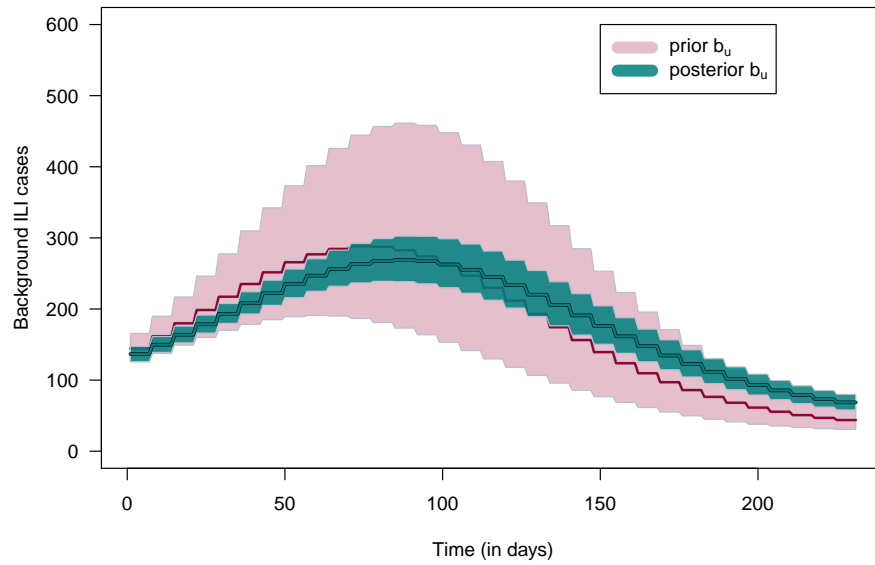

Figure 16: Median (solid line) and 95% CrIs (shaded area) of the prior (red) and posterior (green) for the mean of the rate of the daily number of non-influenza ILI GP consultations.

R Core Team (2018). “R: A Language and Environment for Statistical Computing”. In.

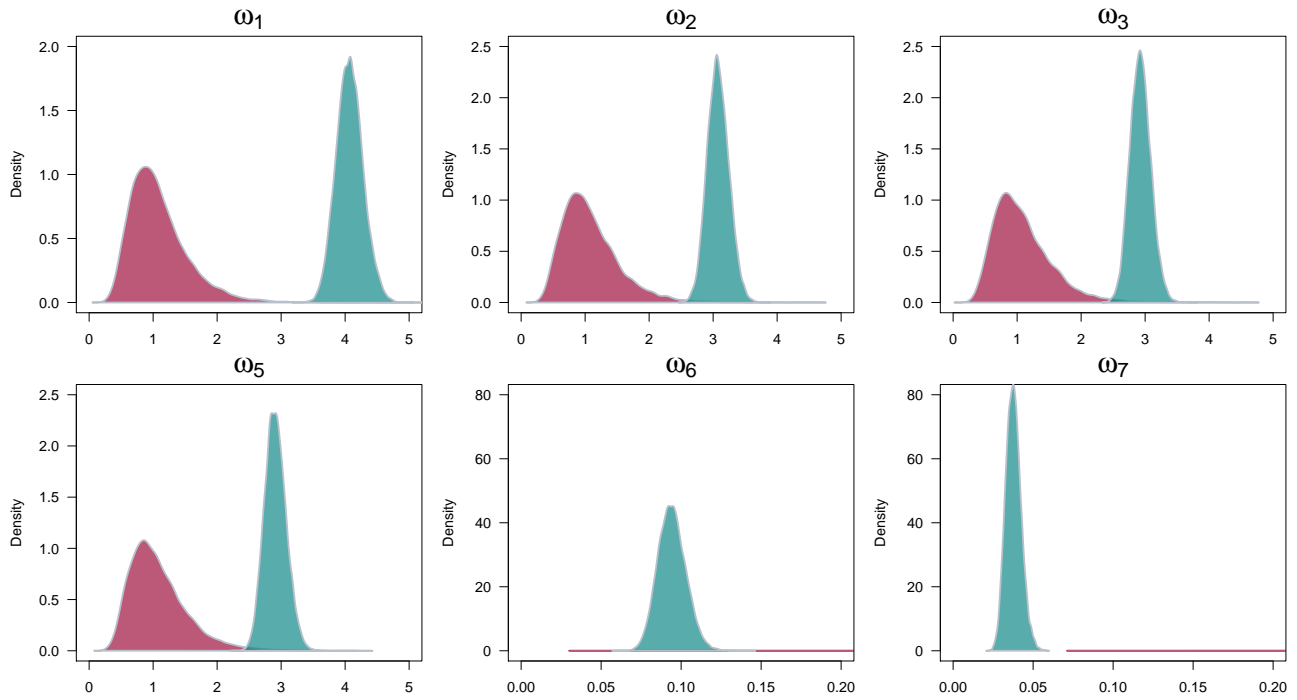

Figure 17: Prior (red) and posterior (green) distributions of the day-of-the-week parameters.

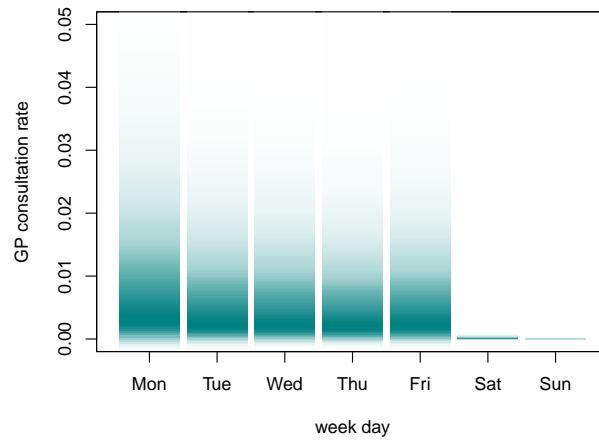

Figure 18: Density strips of the day-specific probability of GP consultation for influenza cases.

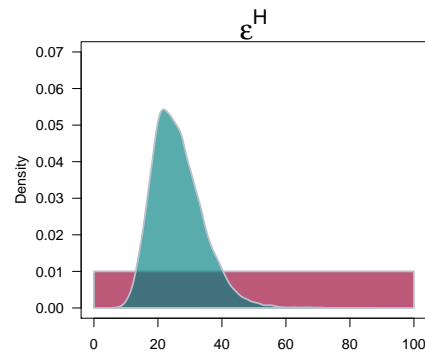

Figure 19: Prior (red) and posterior (green) distributions of the shape parameter of the detection of influenza hospitalizations.

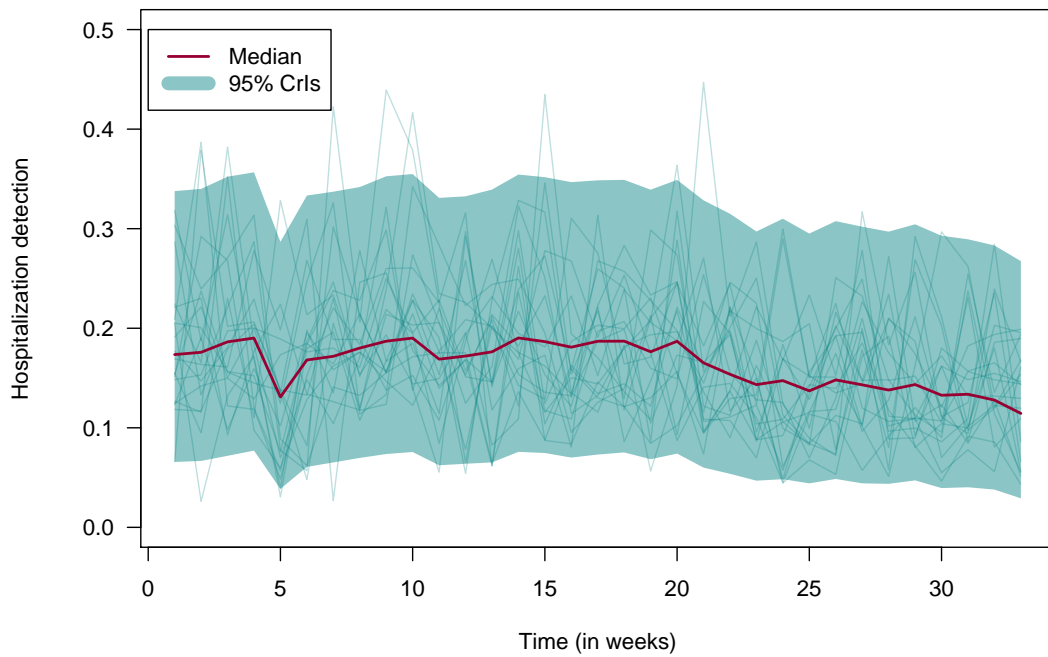

Figure 20: Median (red) and 95% CrIs (green) for the probability of detecting an hospitalised influenza case. 20 trajectories are also simulated and plotted as thin green lines.

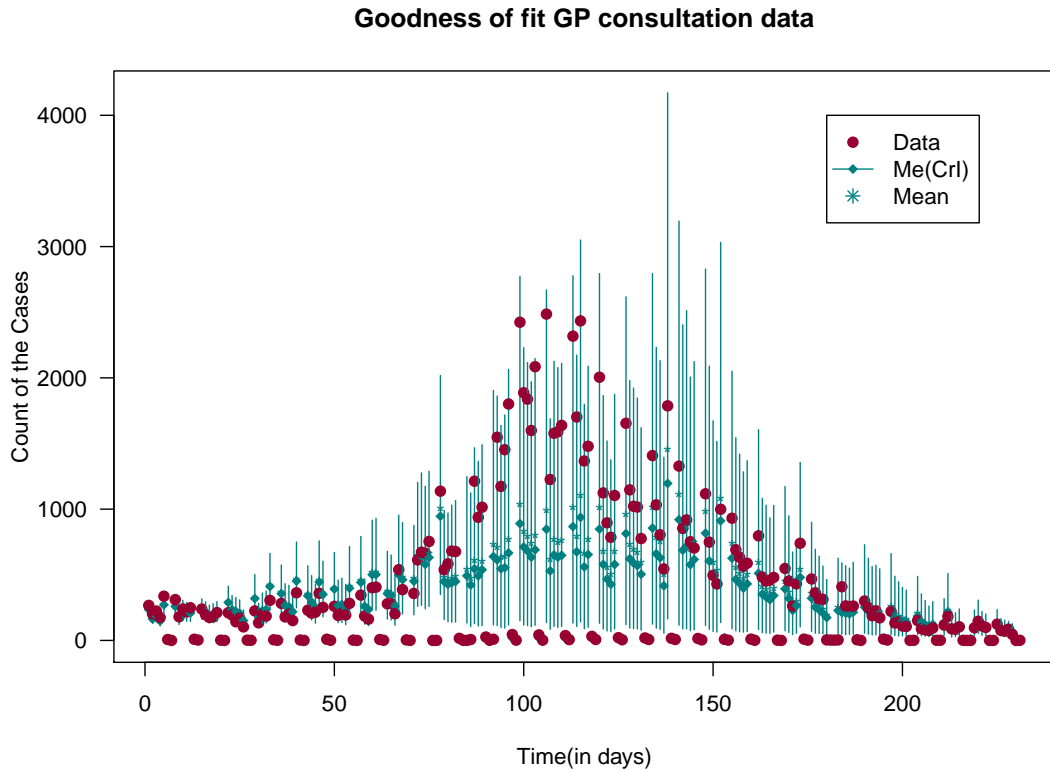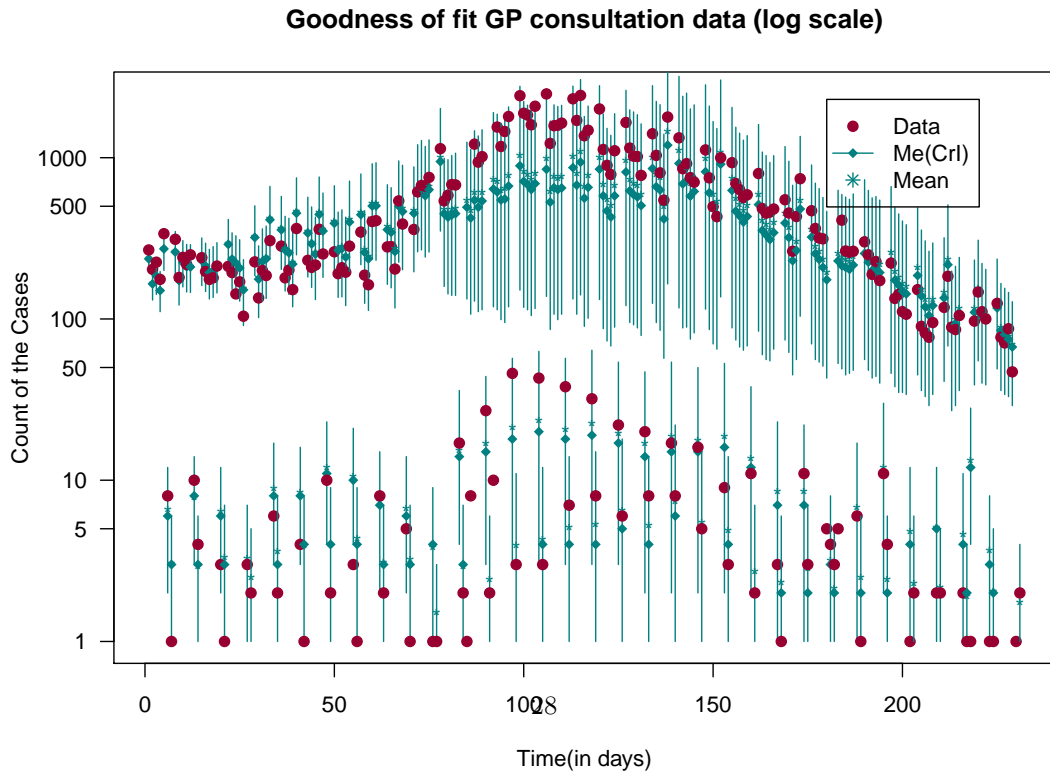

Figure 21: Median and 95% CrIs (green) for the posterior predicted distribution of the number of daily GP consultations on the natural (top panel) and logarithmic (bottom panel) scale. Red points are data.

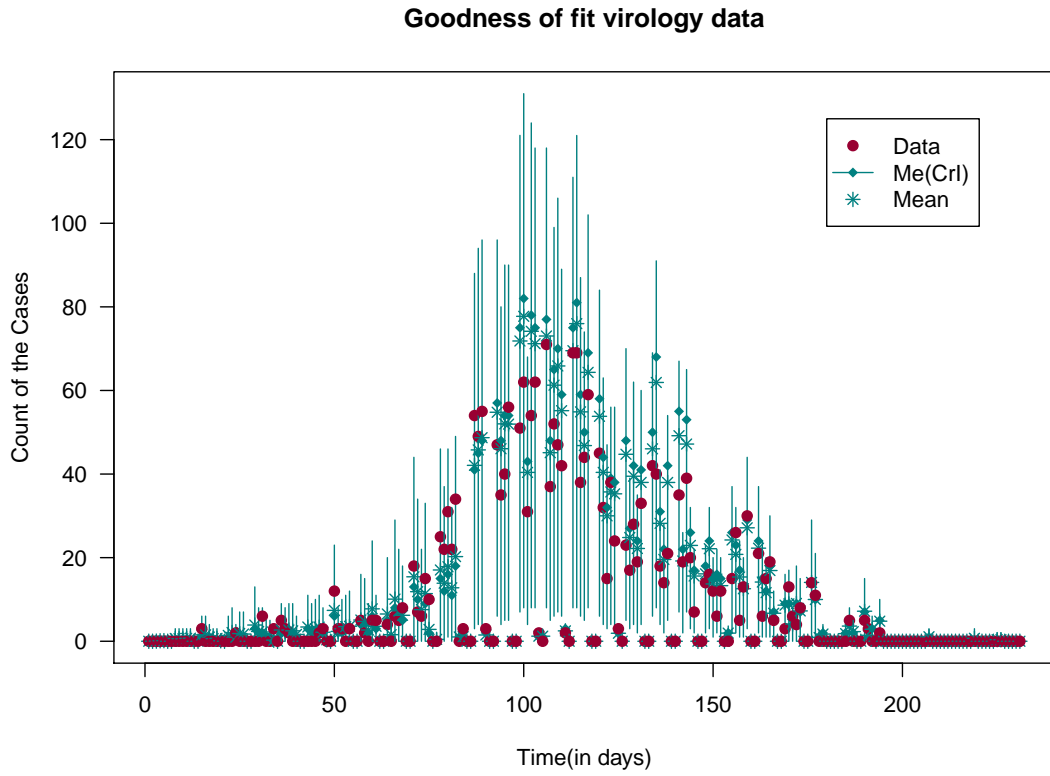

Figure 22: Median and 95% CrIs (green) for the posterior predicted distribution of the number of daily influenza-positive tests. Red points are data.

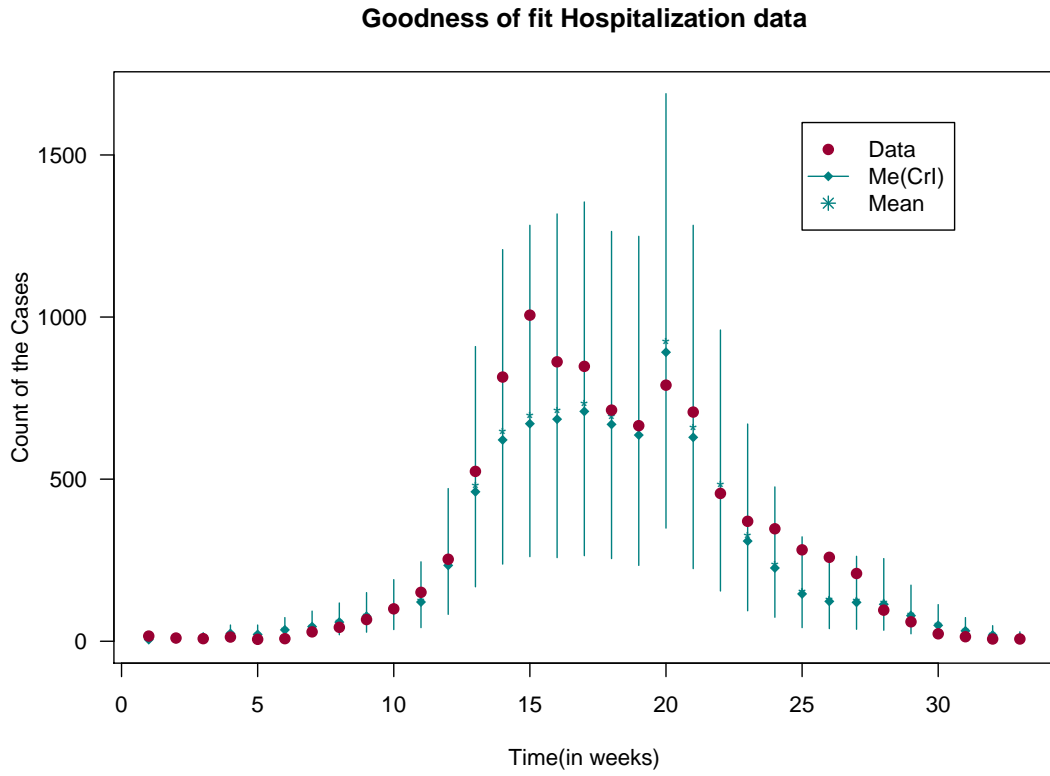

Figure 23: Median and 95% CrIs (green) for the posterior predicted distribution of the number of weekly hospital admissions. Red points are data.

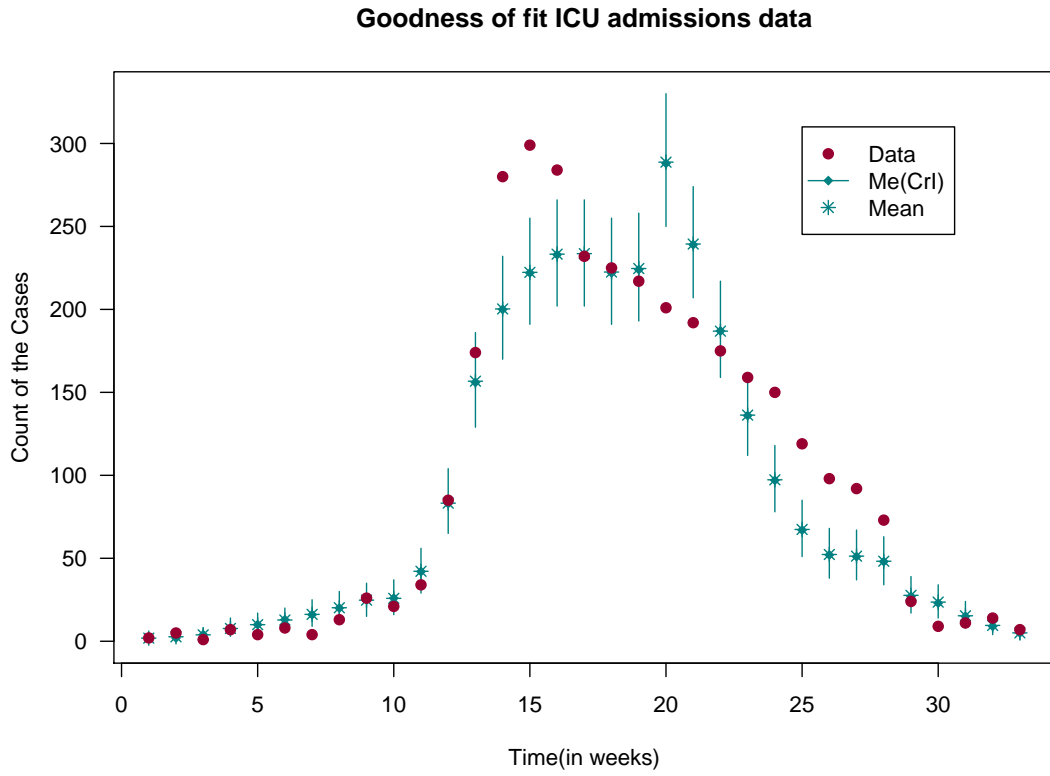

Figure 24: Median and 95% CrIs (green) for the posterior predicted distribution of the number of weekly ICU admissions. Red points are data.
